# Supplementary material for: Predicting Core Electron Binding Energies in Elements of the First Transition Series Using the $\Delta$-Self-Consistent-Field Method
Source: arXiv:2112.04200 source file (2021-12-08)
Supplement: Supplementary file 1 [file Supplementary_information_v3.pdf]

# Supplementary Information for

## Predicting Core Electron Binding Energies in Elements of the First Transition Series Using the Δ-Self-Consistent-Field Method

J. Matthias Kahk[a] and Johannes Lischner[b]

[a] *Institute of Physics, University of Tartu, W. Ostwaldi 1, 50411 Tartu, Estonia*

[b] *Department of Physics and Department of Materials, and the Thomas Young Centre for Theory and Simulation of Materials, Imperial College London, London SW7 2AZ, United Kingdom*

# Table of Contents


Experimental and calculated core electron binding energies....3

Basis set used for Ti atoms with a core hole....5

Basis set used for V atoms with a core hole....7

Basis set used for Cr atoms with a core hole....9

Basis set used for Mn atoms with a core hole....11

Basis set used for Fe atoms with a core hole....13

Basis set used for Co atoms with a core hole....15

Evaluation of the basis sets used in this work....17

Relaxed atomic structures....18

Sample control.in files (excluding the definitions of basis sets) for $MnO_3Cl$....78

# Experimental and calculated core electron binding energies

| Molecule | Experimental binding energy | ΔSCF (Calculated 2p binding energy) | ΔSCF with spin-orbit correction (Calculated $2p_{3/2}$ binding energy) | Error | ΔSCF with spin-orbit correction and element-specific empirical correction (Theoretical best estimate of $2p_{3/2}$ binding energy) | Error after the application of the element-specific empirical correction |
|---|---|---|---|---|---|---|
| $TiF_4$ | 468.60 | 469.17 | 467.04 | -1.56 | 468.21 | -0.39 |
| $TiCl_4$ | 465.40 | 466.67 | 464.53 | -0.87 | 465.70 | 0.30 |
| $TiBr_4$ | 464.40 | 465.83 | 463.70 | -0.70 | 464.87 | 0.47 |
| $TiI_4$ | 463.80 | 464.79 | 462.65 | -1.15 | 463.82 | 0.02 |
| $Ti(NO_3)_4$ | 466.80 | 467.37 | 465.24 | -1.56 | 466.40 | -0.40 |
| $V(CO)_3C_7H_7$ | 519.00 | 520.90 | 518.33 | -0.67 | 519.38 | 0.38 |
| $V(CO)_4C_5H_5$ | 519.80 | 521.64 | 519.07 | -0.73 | 520.12 | 0.32 |
| $VF_5$ | 529.10 | 530.26 | 527.70 | -1.40 | 528.75 | -0.35 |
| $VOCl_3$ | 525.00 | 526.41 | 523.84 | -1.16 | 524.89 | -0.11 |
| $VOF_3$ | 527.30 | 528.58 | 526.01 | -1.29 | 527.06 | -0.24 |
| $Cr(C_5H_5)(CO)_2NO$ | 581.77 | 584.22 | 580.99 | -0.78 | 581.91 | 0.14 |
| $Cr(C_5H_5)(CO)_2NS$ | 581.61 | 583.87 | 580.64 | -0.97 | 581.56 | -0.05 |
| $Cr(C_5H_5)(NO)_2Cl$ | 582.67 | 584.82 | 581.59 | -1.08 | 582.51 | -0.16 |
| $Cr(C_5H_5)(NO)_2NO_2$ | 582.57 | 584.74 | 581.51 | -1.06 | 582.43 | -0.14 |
| $Cr(C_6H_5CH_3)(CO)_3$ | 580.87 | 583.27 | 580.04 | -0.83 | 580.96 | 0.09 |
| $Cr(C_6H_5Cl)(CO)_3$ | 581.17 | 583.37 | 580.14 | -1.03 | 581.06 | -0.11 |
| $Cr(C_6H_6)(CO)_2CS$ | 580.91 | 583.31 | 580.07 | -0.84 | 580.99 | 0.08 |
| $Cr(C_6H_6)(CO)_3$ | 581.08 | 583.43 | 580.20 | -0.88 | 581.12 | 0.04 |
| $Cr(CO)_5C(OCH_3)CH_3$ | 581.61 | 583.63 | 580.39 | -1.22 | 581.31 | -0.30 |
| $Cr(CO)_5CS$ | 581.70 | 584.39 | 581.16 | -0.54 | 582.08 | 0.38 |
| $Cr(CO)_5PF_3$ | 582.04 | 584.53 | 581.29 | -0.75 | 582.21 | 0.17 |
| $Cr(CO)_6$ | 582.00 | 584.62 | 581.39 | -0.61 | 582.31 | 0.31 |
| $CrO_2Cl_2$ | 587.81 | 589.69 | 586.46 | -1.35 | 587.38 | -0.43 |
| $Mn_2(CO)_{10}$ | 647.01 | 650.47 | 646.73 | -0.28 | 647.38 | 0.37 |
| $Mn(CO)_2(CS)C_5H_5$ | 646.77 | 649.56 | 645.83 | -0.94 | 646.48 | -0.29 |
| $Mn(CO)_3C_5H_4CH_3$ | 646.40 | 649.55 | 645.81 | -0.59 | 646.46 | 0.06 |

| | | | | | | |
|---|---|---|---|---|---|---|
| $Mn(CO)_3C_5H_5$ | 646.74 | 649.84 | 646.11 | -0.63 | 646.76 | 0.02 |
| $Mn(CO)_3C_5Me_5$ | 646.08 | 648.89 | 645.16 | -0.92 | 645.81 | -0.27 |
| $Mn(CO)_4NO$ | 647.37 | 650.92 | 647.18 | -0.19 | 647.83 | 0.46 |
| $Mn(CO)_5Br$ | 647.94 | 651.07 | 647.34 | -0.60 | 647.99 | 0.05 |
| $Mn(CO)_5CF_3$ | 648.09 | 650.78 | 647.04 | -1.05 | 647.69 | -0.40 |
| $Mn(CO)_5CH_3$ | 647.10 | 650.40 | 646.67 | -0.43 | 647.32 | 0.22 |
| $Mn(CO)_5Cl$ | 647.98 | 651.01 | 647.28 | -0.70 | 647.93 | -0.05 |
| $Mn(CO)_5COCF_3$ | 647.90 | 650.87 | 647.14 | -0.76 | 647.78 | -0.12 |
| $Mn(CO)_5COCH_3$ | 647.23 | 650.43 | 646.69 | -0.54 | 647.34 | 0.11 |
| $Mn(CO)_5H$ | 647.38 | 650.66 | 646.93 | -0.45 | 647.58 | 0.20 |
| $Mn(CO)_5I$ | 647.73 | 650.96 | 647.23 | -0.50 | 647.87 | 0.14 |
| $Mn(CO)_5SiCl_3$ | 647.84 | 650.74 | 647.00 | -0.84 | 647.65 | -0.19 |
| $Mn(CO)_5SiF_3$ | 648.12 | 651.06 | 647.32 | -0.80 | 647.97 | -0.15 |
| $Mn(NO)_3CO$ | 647.30 | 650.62 | 646.89 | -0.41 | 647.54 | 0.24 |
| $Mn(NO)_3P(CH_3)_3$ | 646.56 | 649.30 | 645.57 | -0.99 | 646.21 | -0.35 |
| $MnO_3Cl$ | 653.41 | 656.44 | 652.71 | -0.70 | 653.36 | -0.05 |
| $Fe(CO)_2(NO)_2$ | 715.58 | 719.36 | 715.00 | -0.58 | 715.48 | -0.10 |
| $Fe(CO)_3C_4H_6$ | 714.82 | 718.73 | 714.37 | -0.45 | 714.85 | 0.03 |
| $Fe(CO)_4C_2H_4$ | 715.40 | 719.30 | 714.93 | -0.47 | 715.41 | 0.01 |
| $Fe(CO)_4H_2$ | 715.97 | 719.81 | 715.44 | -0.53 | 715.92 | -0.05 |
| $Fe(CO)_4P(CH_3)_3$ | 714.74 | 718.53 | 714.16 | -0.58 | 714.64 | -0.10 |
| $Fe(CO)_5$ | 715.85 | 719.86 | 715.49 | -0.35 | 715.97 | 0.13 |
| $Fe(C_5H_5)_2$ | 713.05 | 717.03 | 712.66 | -0.39 | 713.14 | 0.09 |
| $Co_2(CO)_6C_2H_2$ | 786.23 | 790.86 | 785.83 | -0.40 | 786.28 | 0.05 |
| $Co_2(CO)_8$ | 786.34 | 791.27 | 786.23 | -0.11 | 786.69 | 0.35 |
| $Co_3(CO)_9CBr$ | 786.33 | 790.75 | 785.71 | -0.62 | 786.17 | -0.16 |
| $Co_3(CO)_9CCH_3$ | 786.26 | 790.80 | 785.77 | -0.49 | 786.22 | -0.04 |
| $Co_3(CO)_9CCl$ | 786.38 | 790.76 | 785.72 | -0.66 | 786.18 | -0.20 |
| $Co_4(CO)_{12}$ | 785.75 | 790.71 | 785.67 | -0.08 | 786.13 | 0.38 |
| $Co(CO)_2C_5H_5$ | 786.25 | 790.41 | 785.38 | -0.87 | 785.83 | -0.42 |
| $Co(CO)_3NO$ | 786.85 | 791.40 | 786.36 | -0.49 | 786.82 | -0.03 |
| $Co(CO)_4H$ | 786.86 | 791.97 | 786.94 | 0.08 | 787.39 | 0.53 |
| $Co_2(CO)_6(CSiMe_3)_2$ | 785.97 | 790.20 | 785.16 | -0.81 | 785.62 | -0.35 |
| $Co_2(CO)_6(Me_3CCCSiMe_3)$ | 785.92 | 790.39 | 785.36 | -0.56 | 785.81 | -0.11 |

All values are given in eV

## Basis set used for Ti atoms with a core hole

```
################################################################################
#
#  FHI-aims "tight" defaults for the Ti atom (V. Blum, 2009), with additional
#  functions to facilitate the relaxation of the remaining electrons in the
#  presence of a core hole.
#
################################################################################
  species        Ti
#     global species definitions
    nucleus             22
    mass                47.867
#
    l_hartree           6
#
    cut_pot             4.0          2.0  1.0
    basis_dep_cutoff    1e-4
#
    radial_base         48 7.0
    radial_multiplier   5
    angular_grids       specified
      division   0.3263   50
      division   0.7218  110
      division   1.0925  194
      division   1.3188  302
      division   1.4940  434
      division   1.6583  590
#      division   1.8821  770
#      division   2.0961  974
#      division   3.3854 1202
#      outer_grid  974
      outer_grid  590
################################################################################
#
#  Definition of "minimal" basis
#
################################################################################
#     valence basis states
    valence      4  s   2.
    valence      3  p   6.
    valence      3  d   2.
#     ion occupancy
    ion_occ      4  s   1.
    ion_occ      3  p   6.
    ion_occ      3  d   1.
################################################################################
#
#  Suggested additional basis functions. For production calculations,
#  uncomment them one after another (the most important basis functions are
#  listed first).
#
```

```
#  Constructed for dimers: 1.6 A, 1.85 A, 2.5 A, 3.25 A, 4.25 A
#
################################################################################
#  "First tier" - improvements: -396.25 meV to -19.41 meV
     hydro 4 f 8
     hydro 3 d 2.7
     ionic 4 p auto
     hydro 5 g 11.6
     ionic 4 s auto
#  "Second tier" - improvements: -16.30 meV to -2.03 meV
     hydro 3 d 4.4
     hydro 6 h 16
     hydro 4 f 9.4
     hydro 4 p 4.5
     hydro 1 s 0.5
#  "Third tier" - improvements: -6.28 meV to -0.37 meV
     hydro 4 d 6.4
     hydro 4 f 10
     hydro 5 g 12
     hydro 2 p 1.7
     hydro 6 h 16.4
     hydro 4 s 3.8
#  Further basis functions: -0.45 meV and smaller improvements
#     hydro 3 d 8.8
#     hydro 5 p 18
#     hydro 4 f 22.4
#     hydro 5 f 7.2  # -0.16 meV
#     hydro 3 d 2.1  # -0.11 meV
#     hydro 5 g 7.4  # -0.09 meV

# Additional core basis functions to facilitate core hole
hydro 1 s 24.0
hydro 2 s 22.0
hydro 2 p 22.0
hydro 2 p 16.0
hydro 3 s 15.0
hydro 3 p 13.0
hydro 3 d 7.0
```

## Basis set used for V atoms with a core hole

```
################################################################################
#
#  FHI-aims "tight" defaults for the V atom (V. Blum, 2009), with additional
#  functions to facilitate the relaxation of the remaining electrons in the
#  presence of a core hole.
#
################################################################################
  species        V
#     global species definitions
    nucleus             23
    mass                50.9415
#
    l_hartree           6
#
    cut_pot             4.0          2.0  1.0
    basis_dep_cutoff    1e-4
#
    radial_base         49 7.0
    radial_multiplier   5
    angular_grids       specified
      division   0.2753   50
      division   0.6242  110
      division   0.9885  194
      division   1.1666  302
      division   1.3189  434
#      division   1.5211  590
#      division   1.6850  770
#      division   1.8688  974
#      division   3.0666 1202
#      outer_grid  974
      outer_grid  434
################################################################################
#
#  Definition of "minimal" basis
#
################################################################################
#     valence basis states
    valence      4  s   2.
    valence      3  p   6.
    valence      3  d   3.
#     ion occupancy
    ion_occ      4  s   1.
    ion_occ      3  p   6.
    ion_occ      3  d   2.
################################################################################
#
#  Suggested additional basis functions. For production calculations,
#  uncomment them one after another (the most important basis functions are
#  listed first).
#
```

```
#  Constructed for dimers: 1.45 A, 1.65 A, 2.25 A, 3.00 A, 4.00 A
#
################################################################################
#  "First tier" - improvements: -573.19 meV to -17.48 meV
     hydro 4 f 9
     hydro 3 d 3
     ionic 4 p auto
     hydro 5 g 12.8
     ionic 4 s auto
#  "Second tier" - improvements: -21.58 meV to -1.18 meV
     hydro 3 d 5.4
     hydro 5 f 11.2
     hydro 6 h 18.4
     hydro 4 d 7
     hydro 4 f 11.2
     hydro 4 p 5.6
     hydro 5 g 14
     hydro 1 s 0.6
#  "Third tier" - improvements: -0.56 meV to -0.32 meV
#     hydro 3 d 8.8
#     hydro 4 p 7.8
#     hydro 6 h 18.8
#     hydro 4 f 24.8
#     hydro 4 s 4.0
#  "Fourth tier" - improvements: -0.30 meV to -0.09 meV
#     hydro 5 p 12
#     hydro 5 g 15.2
#     hydro 5 f 8
#     hydro 5 p 6.4
#     hydro 4 d 5.2
#     hydro 5 s 7.8
#  Further functions - impr. -0.09 meV and below
#     hydro 3 s 12
#     hydro 6 h 20
#     hydro 5 g 7

# Additional core basis functions to facilitate core hole
hydro 1 s 25.0
hydro 2 s 24.0
hydro 2 p 26.0
hydro 2 p 23.0
hydro 3 s 17.0
hydro 3 s 15.0
hydro 3 p 14.0
hydro 3 d  8.0
hydro 4 p 16.6
hydro 5 f 24.2
```

## Basis set used for Cr atoms with a core hole

```
################################################################################
#
#  FHI-aims "tight" defaults for the Cr atom (V. Blum, 2009), with additional
#  functions to facilitate the relaxation of the remaining electrons in the
#  presence of a core hole.
#
################################################################################
  species        Cr
#     global species definitions
    nucleus             24
    mass                51.9961
#
    l_hartree           6
#
    cut_pot             4.0          2.0  1.0
    basis_dep_cutoff    1e-4
#
    radial_base         50 7.0
    radial_multiplier   5
    angular_grids       specified
      division   0.2623   50
      division   0.5927  110
      division   0.9348  194
      division   1.1233  302
      division   1.2671  434
#      division   1.4867  590
#      division   1.7111  770
#      division   1.9339  974
#      division   2.8695 1202
#      outer_grid  974
      outer_grid  590
################################################################################
#
#  Definition of "minimal" basis
#
################################################################################
#     valence basis states
    valence      4  s   2.
    valence      3  p   6.
    valence      3  d   4.
#     ion occupancy
    ion_occ      4  s   1.
    ion_occ      3  p   6.
    ion_occ      3  d   3.
################################################################################
#
#  Suggested additional basis functions. For production calculations,
#  uncomment them one after another (the most important basis functions are
#  listed first).
#
```

```
#  Constructed for dimers: 1.375 A, 1.55 A, 2.00 A, 2.75 A, 3.75 A
#
################################################################################
#  "First tier" - improvements: -633.53 meV to -21.19 meV
     hydro 4 f 9.6
     hydro 3 d 3.1
     ionic 4 p auto
     hydro 5 g 13.6
     ionic 4 s auto
#  "Second tier" - improvements: -23.49 meV to -1.88 meV
     hydro 4 f 6.8
     hydro 4 d 14.4
     hydro 6 h 19.2
     ionic 3 d auto
     hydro 4 f 14.8
     hydro 5 g 10.4
     hydro 1 s 0.6
     hydro 3 p 3.5
#  "Third tier" - improvements: -1.02 meV to -0.20 meV
#     hydro 6 h 15.6
#     hydro 3 d 7.4
#     hydro 4 p 18.4
#     hydro 5 g 16.4
#     hydro 4 s 3.9
#     hydro 4 f 28.8
#  "Fourth tier" - improvements: -0.42 meV to -0.09 meV
#     hydro 4 d 10.4
#     hydro 5 p 7
#     hydro 4 s 20
#     hydro 5 f 7.2
#     hydro 5 g 20.4
#     hydro 6 h 16.8
#  Further functions: improvements -0.07 meV and below
#     hydro 5 f 30
#     hydro 5 p 17.2
#     hydro 3 s 2.2
#     hydro 5 s 7.6

# Additional core basis functions to facilitate core hole
hydro 1 s 26.0
hydro 2 s 25.0
hydro 2 p 27.0
hydro 2 p 24.0
hydro 3 s 18.0
hydro 3 s 16.0
hydro 3 p 15.0
hydro 3 d  9.0
hydro 4 p 17.6
hydro 5 f 25.2
```

## Basis set used for Mn atoms with a core hole

```
################################################################################
#
#  FHI-aims "tight" defaults for the Mn atom (V. Blum, 2009), with additional
#  functions to facilitate the relaxation of the remaining electrons in the
#  presence of a core hole.
#
################################################################################
  species        Mn
#     global species definitions
    nucleus             25
    mass                54.938045
#
    l_hartree           6
#
    cut_pot             4.0          2.0  1.0
    basis_dep_cutoff    1e-4
#
    radial_base         50 7.0
    radial_multiplier   5
    angular_grids       specified
      division   0.2623   50
      division   0.5927  110
      division   0.9156  194
      division   1.1008  302
      division   1.2671  434
#      division   1.5167  590
#      division   1.7111  770
#      division   1.8945  974
#      division   2.7372 1202
      outer_grid  590
################################################################################
#
#  Definition of "minimal" basis
#
################################################################################
#     valence basis states
    valence      4  s   2.
    valence      3  p   6.
    valence      3  d   5.
#     ion occupancy
    ion_occ      4  s   1.
    ion_occ      3  p   6.
    ion_occ      3  d   4.
################################################################################
#
#  Suggested additional basis functions. For production calculations,
#  uncomment them one after another (the most important basis functions are
#  listed first).
#
#  Constructed for dimers: 1.40 A, 1.60 A, 2.10 A, 2.75 A, 3.75 A
```

```
#
################################################################################
#  "First tier" - improvements: -466.21 meV to -15.27 meV
     hydro 4 f 9.6
     hydro 3 d 3.2
     hydro 2 p 2
     hydro 5 g 13.6
     hydro 3 s 3.3
#  "Second tier" - improvements: -21.45 meV to -1.55 meV
     hydro 3 d 6
     hydro 6 h 19.2
     hydro 4 f 6.4
     hydro 4 f 17.2
     hydro 3 p 3.1
     hydro 3 d 6.2
     hydro 5 g 10.8
     hydro 3 s 3.8
#  "Third tier" - improvements: -1.38 meV to -0.13 meV
#     hydro 5 p 8.6   -1.38 meV
#     hydro 6 h 16    -0.73 meV
#     hydro 3 d 10.8  -0.43 meV
#     hydro 5 f 6.8   # forced: -0.26 meV
#     hydro 5 g 6.4   # forced: -0.21 meV
#     hydro 5 s 9.8   # forced: -0.13 meV
#  Further functions: improvements -0.32 meV and below
#     hydro 3 p 19.6  # -0.32 meV
#     hydro 5 f 28.4  # -0.20 meV
#     hydro 4 f 26    # -0.08 meV
#     hydro 3 p 3.5
#     hydro 5 g 14.8
#     hydro 5 s 9
#     hydro 4 p 16.8
#     hydro 6 h 18
#     hydro 4 d 13.6
# Additional core basis functions to facilitate core hole
hydro 1 s 27.0
hydro 2 s 26.0
hydro 2 p 28.0
hydro 2 p 25.0
hydro 3 s 19.0
hydro 3 s 17.0
hydro 3 p 16.0
hydro 3 d 10.0
hydro 4 p 18.6
hydro 5 f 26.2
```

## Basis set used for Fe atoms with a core hole

```
################################################################################
#
#  FHI-aims "tight" defaults for the Fe atom (V. Blum, 2009), with additional
#  functions to facilitate the relaxation of the remaining electrons in the
#  presence of a core hole.
#
################################################################################
  species        Fe
#     global species definitions
    nucleus             26
    mass                55.845
#
    l_hartree           6
#
    cut_pot             4.0          2.0  1.0
    basis_dep_cutoff    0.0
#
    radial_base         51 7.0
    radial_multiplier   4
    angular_grids       specified
      division   0.2739   50
      division   0.5898  110
      division   0.9223  194
      division   1.1267  302
      division   1.3186  434
#      division   1.5125  590
#      division   1.7365  770
#      division   1.9990  974
#      division   2.7593 1202
#      outer_grid  1202
      outer_grid  434
################################################################################
#
#  Definition of "minimal" basis
#
################################################################################
#     valence basis states
    valence      4  s   2.
    valence      3  p   6.
    valence      3  d   6.
#     ion occupancy
    ion_occ      4  s   1.
    ion_occ      3  p   6.
    ion_occ      3  d   5.
################################################################################
#
#  Suggested additional basis functions. For production calculations,
#  uncomment them one after another (the most important basis functions are
#  listed first).
#
```

```
#  Constructed for dimers: 1.45 A, 1.725 A, 2.25 A, 3.00 A, 4.00 A
#
################################################################################
#  "First tier" - improvements: -300.53 meV to -10.50 meV
     hydro 4 f 9.4
     hydro 2 p 2.2
     hydro 5 g 12.4
     hydro 3 d 3.1
     ionic 4 s auto
#  "Second tier" - improvements: -16.31 meV to -0.65 meV
     hydro 3 d 6.2
     hydro 6 h 19.2
     hydro 4 f 15.2
     hydro 4 f 6.6
     hydro 3 p 3
     hydro 5 g 13.2
     hydro 1 s 0.65
#  "Third tier" - improvements: -1.60 meV to -0.10 meV
#     hydro 4 d 7.8
#     hydro 4 p 19.6
#     hydro 4 d 10.4
#     ionic 4 p auto
#     hydro 6 h 17.6
#     hydro 5 f 27.2
#     hydro 4 s 4.8
#  "Fourth tier": improvements -0.13 meV and below
#     hydro 5 f 12
#     hydro 5 g 10.4
#     hydro 5 p 8.4
#     hydro 4 d 14.8
#     hydro 2 s 1.9

# Additional core basis functions to facilitate core hole
hydro 2 s 27.0
hydro 2 p 29.0
hydro 2 p 26.0
hydro 3 s 20.0
hydro 3 s 18.0
hydro 3 p 17.0
hydro 3 d 11.0
hydro 4 p 19.6
hydro 5 f 27.2
```

## Basis set used for Co atoms with a core hole

```
################################################################################
#
#  FHI-aims "tight" defaults for the Co atom (V. Blum, 2009), with additional
#  functions to facilitate the relaxation of the remaining electrons in the
#  presence of a core hole.
#
################################################################################
  species        Co
#     global species definitions
    nucleus      27
    mass         58.933195
#
    l_hartree    6
#
    cut_pot      4.0  2.0  1.0
    basis_dep_cutoff    1e-4
#
    radial_base        52 7.0
    radial_multiplier  2
    angular_grids       specified
      division   0.3189   50
      division   0.6267  110
      division   0.9473  194
      division   1.1520  302
      division   1.3966  434
#      division   1.6293  590
#      division   1.8317  770
#      division   2.0231  974
#      division   2.4367 1202
#      outer_grid   974
      outer_grid  434
################################################################################
#
#  Definition of "minimal" basis
#
################################################################################
#     valence basis states
    valence      4  s   2.
    valence      3  p   6.
    valence      3  d   7.
#     ion occupancy
    ion_occ      4  s   1.
    ion_occ      3  p   6.
    ion_occ      3  d   6.
################################################################################
#
#  Suggested additional basis functions. For production calculations,
#  uncomment them one after another (the most important basis functions are
#  listed first).
#
```

```
#  Constructed for dimers: 1.8, 2.0, 2.5, 3.5 Ang
#
################################################################################
#  "First tier" (improvements: -167.79 meV ...  -15.31 meV)
     hydro 3 p 5.8
     hydro 4 f 8.2
     hydro 3 d 5.4
     hydro 5 g 12
     ionic 4 s auto
#  "Second tier" (improvements: -8.83 meV ... -0.89 meV)
     ionic 4 p auto
     hydro 6 h 16.4
     hydro 4 d 5.6
#     hydro 4 f 17.2
#     hydro 1 s 0.75
#  "Third tier" (improvements: -1.03 meV ... -0.06 meV)
#     hydro 4 d 7.8
#     hydro 2 p 5.8
#     hydro 4 f 8
#     hydro 5 g 11.6
#     hydro 4 s 4.3
#     hydro 6 h 14.4
#  "Fourth tier" (minor improvements)
#     hydro 5 f 16
#     hydro 5 d 8
#     hydro 4 p 10
#     hydro 5 s 7.4

# Additional core basis functions to facilitate core hole
hydro 2 s 28.0
hydro 2 p 30.0
hydro 2 p 27.0
hydro 3 s 21.0
hydro 3 s 19.0
hydro 3 p 18.0
hydro 3 d 12.0
hydro 4 p 20.6
hydro 5 f 28.2
```

## Evaluation of the basis sets used in this work

In ΔSCF calculations of core electron binding energies, on the atom with a core hole it is important to use a basis set that is able to accommodate the relaxation of both the remaining core and valence electrons in the final state with a missing core electron. In this work, in line with our previous studies, basis sets with variational freedom for the core electrons have been constructed by adding additional tight basis functions to the default atom-centered numerical basis sets of FHI-aims. Another way for constructing basis sets with a high degree of variational freedom for the core orbitals is by uncontracting optimized all-electron Gaussian basis sets. In order to verify that the two different strategies ultimately yield similar results, we have performed an additional set of ΔSCF calculations: TM $2p_{3/2}$ core electron binding energies in $TiCl_4$, $VOCl_3$, $Cr(CO)_6$, $Mn(CO)_5H$, $Fe(CO)_5$, and $Co(CO)_4H$ have been calculated in both FHI-aims and NWChem, using numerical basis sets and Gaussian basis sets respectively. In order to obtain comparable results, non-relativistic calculations have been performed in both codes, and DFT with the PBE exchange-correlation functional has been used. In the NWChem calculations, uncontracted forms of the "polarization-consistent" pc-3 basis sets from *J. Chem. Phys.* **138**, 014107 (2013) were used for the atoms with a core hole, and regular pc-3 basis sets were used for all other atoms. The results are shown in the table below – all values are given in eV.

| | $TiCl_4$ | $VOCl_3$ | $Cr(CO)_6$ | $Mn(CO)_5H$ | $Fe(CO)_5$ | $Co(CO)_4H$ |
|---|---|---|---|---|---|---|
| Ground $E_{tot}$ (numerical basis) | -73191.49 | -65290.32 | -46913.47 | -46745.68 | -49797.06 | -49970.21 |
| Ground $E_{tot}$ (u-pc-3) | -73191.43 | -65290.28 | -46913.47 | -46745.67 | -49797.05 | -49970.21 |
| Ground $E_{tot}$ (difference) | -0.06 | -0.05 | -0.01 | -0.01 | -0.01 | 0.00 |
| Hole $E_{tot}$ (numerical basis) | -72728.42 | -64768.04 | -46333.13 | -46099.96 | -49082.78 | -49184.50 |
| Hole $E_{tot}$ (u-pc-3) | -72728.44 | -64767.98 | -46333.13 | -46099.97 | -49082.81 | -49184.55 |
| Hole $E_{tot}$ (difference) | 0.02 | -0.06 | -0.01 | 0.01 | 0.03 | 0.05 |
| ΔSCF (numerical basis) | 463.07 | 522.28 | 580.34 | 645.72 | 714.27 | 785.70 |
| ΔSCF (u-pc-3) | 462.99 | 522.30 | 580.34 | 645.70 | 714.24 | 785.65 |
| ΔSCF (difference) | 0.08 | -0.01 | 0.00 | 0.02 | 0.03 | 0.05 |

In all cases, the core electron binding energies from the two different sets of calculations agree with each other to within 0.1 eV. This indicates that although some further optimization of the numerical basis sets used in this work may be possible, basis set incompleteness cannot be the primary reason for the systematic underestimation of core electron binding energies observed in this study. We emphasize that the results of the nonrelativistic calculations are only presented for the evaluation of basis sets and other numerical details, they have not been adjusted for spin-orbit splittings, and cannot therefore be directly compared to experiment.

# Relaxed atomic structures

## $Co_2(CO)_6C_2H_2$

18
Atoms.

| | | | |
|---|---|---|---|
| Co | 0.1081296 | 0.0761112 | 0.0173467 |
| Co | 2.5541329 | 0.1015518 | 0.0252511 |
| C | -1.3765464 | 0.9958693 | 0.0355771 |
| C | 1.3150572 | 1.4189784 | 0.7197423 |
| C | 1.3191888 | 1.4480294 | -0.6193410 |
| O | -2.3357547 | 1.6114432 | 0.0484878 |
| H | 1.3150018 | 2.1312733 | -1.4506568 |
| C | -0.1654682 | -0.9818309 | 1.4222792 |
| C | -0.1575658 | -0.9168741 | -1.4358020 |
| O | -0.3344099 | -1.6399630 | 2.3363324 |
| O | -0.3204262 | -1.5324638 | -2.3800780 |
| C | 4.0194093 | 1.0511408 | 0.0505506 |
| C | 2.8402783 | -0.9484267 | 1.4339162 |
| C | 2.8482238 | -0.8877375 | -1.4249263 |
| O | 4.9659856 | 1.6859075 | 0.0678134 |
| O | 3.0169501 | -1.6017739 | 2.3499103 |
| O | 3.0291143 | -1.5014037 | -2.3671600 |
| H | 1.3054893 | 2.0651986 | 1.5801068 |

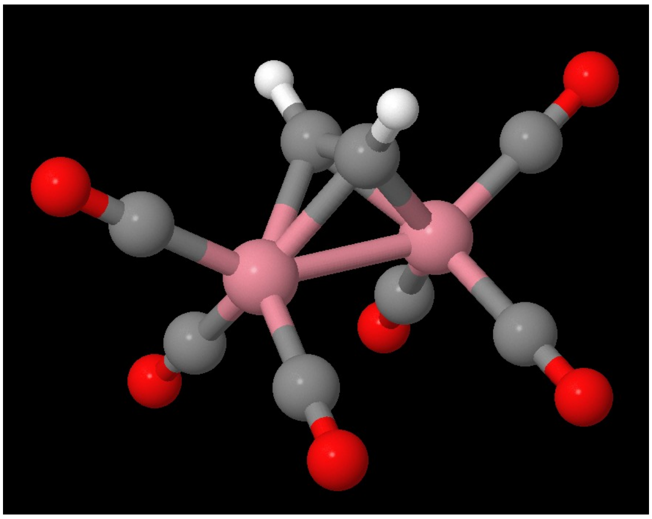

## $Co_2(CO)_6(CSiMe_3)_2$

```
42
Atoms.
Co          0.1199310     -0.0378045      0.0516370
Co          2.5739052      0.0156605     -0.0177459
C          -1.3912927      0.8086089      0.2477515
C           1.3381223      1.3683912      0.7206090
C           1.2966549      1.4012392     -0.6170140
O          -2.3785203      1.3671682      0.3791562
Si          1.2239091      2.4548121     -2.1393736
C          -0.0043301     -1.1861353      1.3962906
C          -0.2242371     -0.9338704     -1.4422725
O          -0.0954505     -1.9328730      2.2538202
O          -0.4774515     -1.4993084     -2.4003352
C           4.0485368      0.9317425     -0.1749041
C           2.9557370     -0.9383034      1.4305945
C           2.7441853     -1.0604304     -1.4162731
O           5.0122228      1.5348062     -0.2824038
O           3.2310835     -1.5412082      2.3592374
O           2.8645123     -1.7615609     -2.3080435
Si          1.3755347      2.3535427      2.2889387
C           1.6692626      1.4331253     -3.6305056
C           2.4375660      3.8591123     -1.9227613
C          -0.5148425      3.1173364     -2.2957464
C           3.0786280      3.1018620      2.4511582
C           1.0036141      1.2451240      3.7374444
C           0.0871337      3.6999929      2.1484425
H           0.0794936      4.3178971      3.0481447
H          -0.9143191      3.2885303      2.0208863
H           0.2916875      4.3534866      1.2992890
H           3.1237477      3.7631561      3.3182375
H           3.3429492      3.6880841      1.5701709
H           3.8398429      2.3319233      2.5805484
H          -0.0067884      0.8394796      3.6793441
H           1.0806558      1.8066668      4.6701374
H           1.6972441      0.4065180      3.7987541
H          -0.5842262      3.8130039     -3.1338548
H          -0.8244189      3.6482996     -1.3947946
H          -1.2300937      2.3132442     -2.4717879
H           2.1865946      4.4676513     -1.0530244
H           2.4271193      4.5107599     -2.7983366
H           3.4567958      3.4940976     -1.7941934
H           1.5640495      2.0280198     -4.5394715
H           1.0256988      0.5591778     -3.7322373
H           2.7010227      1.0838740     -3.5822431
```

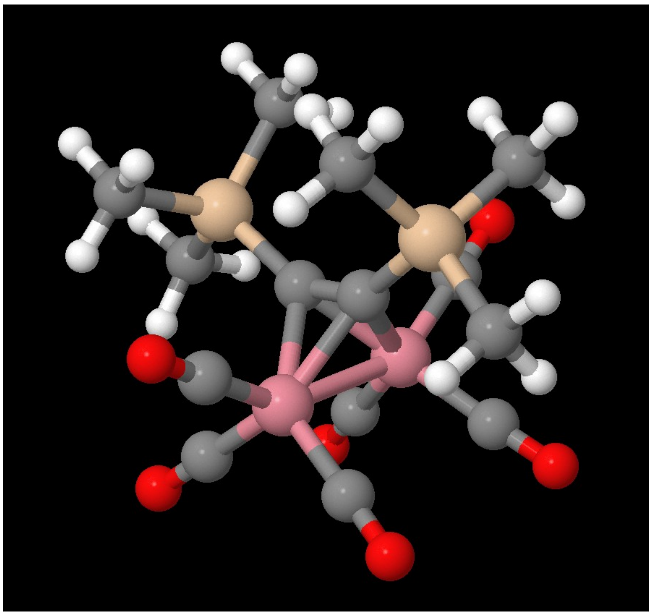

**$Co_2(CO)_6(Me_3CCCSiMe_3)$**

42
Atoms.

| | | | |
|---|---|---|---|
| Co | 0.0855526 | 0.0455297 | 0.1641303 |
| Co | 2.5294305 | 0.0240810 | 0.0954166 |
| C | -1.4247827 | 0.8956121 | 0.3481393 |
| C | 1.3400478 | 1.3758233 | 0.8775559 |
| C | 1.3018720 | 1.4715298 | -0.4591475 |
| O | -2.4291270 | 1.4289974 | 0.4562093 |
| Si | 1.2536984 | 2.5328226 | -1.9750322 |
| C | -0.0625168 | -1.1292208 | 1.4815837 |
| C | -0.2837376 | -0.8202660 | -1.3470047 |
| O | -0.1567374 | -1.8898658 | 2.3265214 |
| O | -0.5490049 | -1.3620229 | -2.3152001 |
| C | 4.0234682 | 0.8967159 | -0.1119208 |
| C | 2.9210490 | -0.9541232 | 1.5242817 |
| C | 2.6592173 | -1.0652849 | -1.3022569 |
| O | 5.0026369 | 1.4642683 | -0.2661385 |
| O | 3.2054247 | -1.5748722 | 2.4382617 |
| O | 2.7482547 | -1.7746506 | -2.1909860 |
| C | 1.3833551 | 2.2406023 | 2.1010634 |
| C | 1.7284503 | 1.5122623 | -3.4589434 |
| C | 2.4611041 | 3.9450086 | -1.7625147 |
| C | -0.4827697 | 3.1919800 | -2.1728214 |
| H | -0.5310662 | 3.8852908 | -3.0145064 |
| H | -0.8189056 | 3.7246097 | -1.2827107 |
| H | -1.1906380 | 2.3853885 | -2.3664219 |
| H | 2.1851787 | 4.5918046 | -0.9290631 |
| H | 2.4802971 | 4.5595414 | -2.6647645 |
| H | 3.4754785 | 3.5850712 | -1.5878588 |
| H | 1.6396583 | 2.1068728 | -4.3698152 |
| H | 1.0888340 | 0.6369236 | -3.5730867 |
| H | 2.7599305 | 1.1650776 | -3.3907020 |
| C | 2.7805620 | 2.8588349 | 2.2127740 |
| C | 1.0760004 | 1.4459313 | 3.3637993 |
| C | 0.3550084 | 3.3642475 | 1.9379051 |
| H | 0.3907436 | 4.0241067 | 2.8052629 |
| H | -0.6560705 | 2.9686306 | 1.8594696 |
| H | 0.5640539 | 3.9571157 | 1.0476281 |
| H | 2.8037132 | 3.5599554 | 3.0475203 |
| H | 3.0462222 | 3.3987754 | 1.3039185 |
| H | 3.5331683 | 2.0919104 | 2.3907265 |
| H | 0.0652888 | 1.0404296 | 3.3332930 |
| H | 1.1564792 | 2.0912461 | 4.2387972 |
| H | 1.7726478 | 0.6182090 | 3.4898972 |

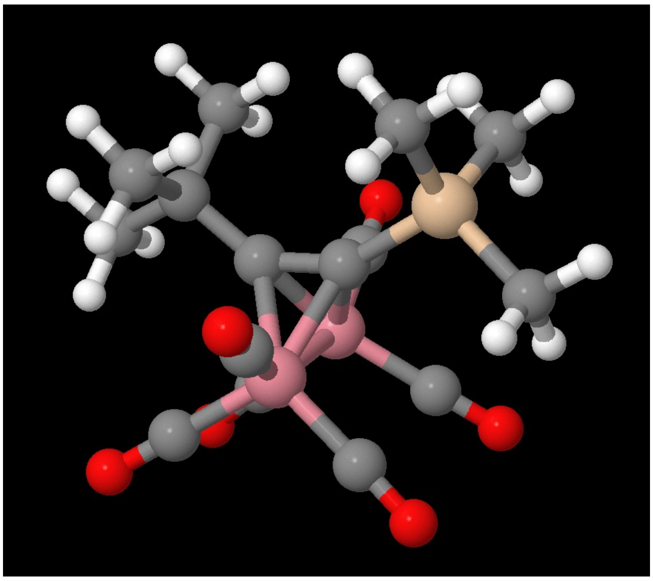

## $Co_2(CO)_8$

```
18
Atoms.
Co          0.0764665     0.0597701    -0.0052228
Co          2.5848514     0.0604721     0.0051707
C          -0.9352410     1.5140162     0.0080469
C           1.3248396     0.7075277     1.3122945
C           1.3361822     0.7366865    -1.2973846
O          -1.6265005     2.4172401     0.0155280
O           1.3204677     1.1876545     2.3702209
O           1.3401759     1.2393936    -2.3447942
C          -0.5578537    -1.0078705     1.2778910
C          -0.5478830    -0.9766498    -1.3184134
O          -0.9838336    -1.6721019     2.0963035
O          -0.9676455    -1.6229794    -2.1541715
C           3.5962672     1.5150180     0.0253721
C           3.2096624    -1.0057518     1.2941833
C           3.2196767    -0.9775174    -1.3017065
O           4.2878777     2.4179092     0.0374421
O           3.6295216    -1.6712168     2.1147360
O           3.6462684    -1.6235105    -2.1342759
```

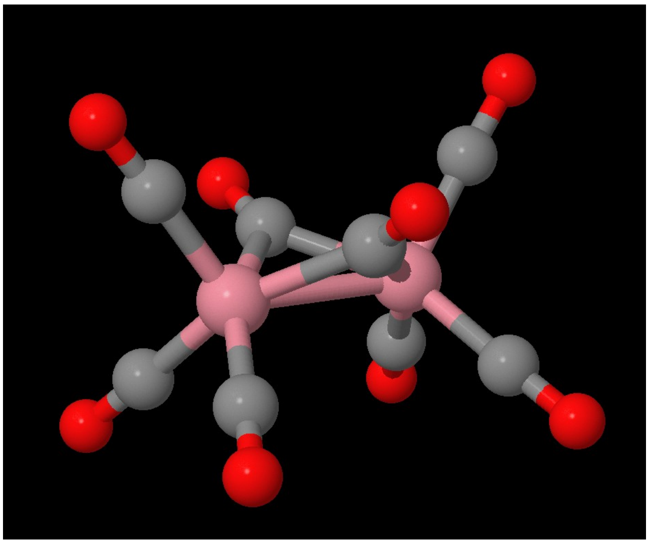

## $Co_3(CO)_9CBr$

```
23
Atoms.
Co          2.0619335      -0.7090774       2.1370843
Co          0.0688685      -1.6340339       3.2310448
Co          2.0728873      -3.0260592       2.9508772
C           1.5875727      -0.9973216       0.4262113
C           1.8169236      -1.4100392       3.8518639
C           1.6972446       0.9878632       2.3940459
C           3.8019996      -0.5077669       2.0536589
C          -0.8412720      -2.1699633       1.7749478
C          -0.6624759      -2.5435414       4.5415043
C          -0.6779515      -0.1012878       3.6410283
C           1.6371829      -3.8479935       1.4117805
C           3.8126751      -3.2255742       3.0607388
C           1.6781503      -4.2131056       4.1804990
O           1.2798942      -1.1850229      -0.6532521
O           1.4937708       2.0942608       2.5684077
O           4.9282579      -0.3473758       2.0086065
O          -1.4091149      -2.5116406       0.8497713
O          -1.1449537      -3.1037067       5.4071295
O          -1.1729541       0.8808841       3.9352021
O           1.3560844      -4.3570186       0.4334565
O           4.9370730      -3.3719115       3.1619626
O           1.4526034      -4.9850304       4.9863917
Br          2.4587730      -0.8192462       5.5227533
```

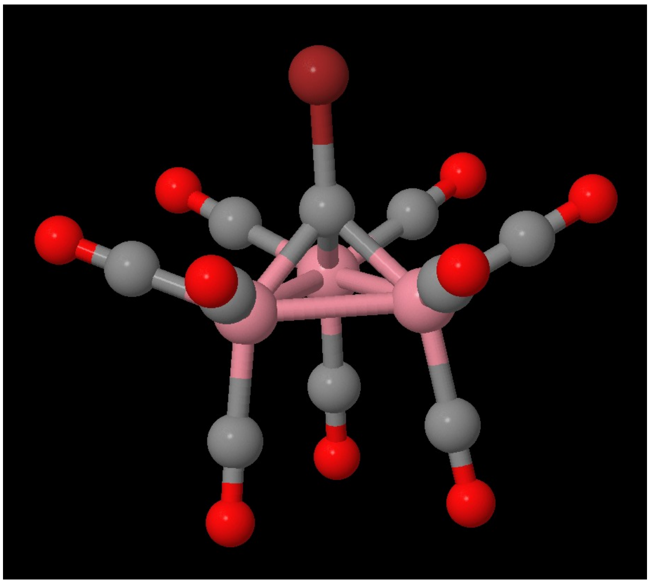

**$Co_3(CO)_9CCH_3$**

26
Atoms.

| | | | |
|---|---|---|---|
| Co | 2.0613887 | -0.7106895 | 2.1411446 |
| Co | 0.0731517 | -1.6336074 | 3.2329257 |
| Co | 2.0724542 | -3.0221112 | 2.9528191 |
| C | 1.5871584 | -0.9975595 | 0.4320266 |
| C | 1.8276024 | -1.4003607 | 3.8791934 |
| C | 1.6980404 | 0.9778108 | 2.4078770 |
| C | 3.7955746 | -0.5126629 | 2.0649536 |
| C | -0.8363343 | -2.1699771 | 1.7791452 |
| C | -0.6461229 | -2.5379712 | 4.5443700 |
| C | -0.6649456 | -0.1044631 | 3.6438051 |
| C | 1.6380440 | -3.8432361 | 1.4151468 |
| C | 3.8058992 | -3.2125219 | 3.0690100 |
| C | 1.6782687 | -4.1998283 | 4.1820859 |
| O | 1.2802958 | -1.1838293 | -0.6484221 |
| O | 1.4992065 | 2.0852515 | 2.5937324 |
| O | 4.9236370 | -0.3490316 | 2.0287328 |
| O | -1.4057772 | -2.5116286 | 0.8543745 |
| O | -1.1222850 | -3.0933303 | 5.4191845 |
| O | -1.1561839 | 0.8794256 | 3.9459688 |
| O | 1.3577583 | -4.3539755 | 0.4369244 |
| O | 4.9318964 | -3.3541022 | 3.1812566 |
| O | 1.4571175 | -4.9686944 | 4.9948272 |
| C | 2.3310359 | -0.9374095 | 5.1894312 |
| H | 1.9789745 | 0.0724477 | 5.4124645 |
| H | 3.4231799 | -0.9213956 | 5.2086285 |
| H | 1.9932432 | -1.5933225 | 5.9951273 |

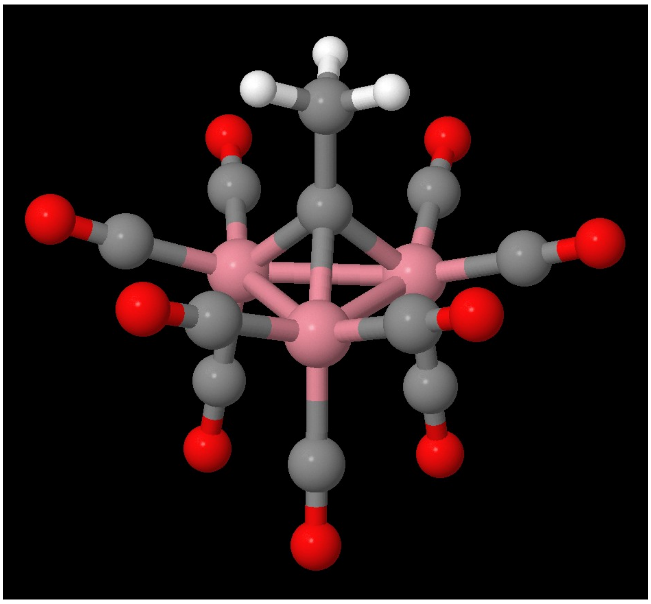

**$Co_3(CO)_9CCl$**

23
Atoms.

| | | | |
|---|---|---|---|
| Co | 2.0620802 | -0.7088171 | 2.1372452 |
| Co | 0.0688124 | -1.6339011 | 3.2314716 |
| Co | 2.0730976 | -3.0260871 | 2.9512637 |
| C | 1.5870266 | -0.9981708 | 0.4266788 |
| C | 1.8185315 | -1.4085390 | 3.8559204 |
| C | 1.6977417 | 0.9875884 | 2.3939156 |
| C | 3.8015078 | -0.5072767 | 2.0537520 |
| C | -0.8401645 | -2.1701397 | 1.7746769 |
| C | -0.6625849 | -2.5429110 | 4.5413945 |
| C | -0.6780338 | -0.1018622 | 3.6414283 |
| C | 1.6367141 | -3.8469018 | 1.4116839 |
| C | 3.8122037 | -3.2258972 | 3.0612187 |
| C | 1.6786593 | -4.2130026 | 4.1802395 |
| O | 1.2797155 | -1.1851392 | -0.6530424 |
| O | 1.4941559 | 2.0943511 | 2.5670563 |
| O | 4.9278639 | -0.3466175 | 2.0075855 |
| O | -1.4086611 | -2.5117564 | 0.8498491 |
| O | -1.1461648 | -3.1034076 | 5.4064365 |
| O | -1.1741035 | 0.8801454 | 3.9350507 |
| O | 1.3561034 | -4.3565362 | 0.4335083 |
| O | 4.9367351 | -3.3731724 | 3.1616983 |
| O | 1.4530189 | -4.9859609 | 4.9853697 |
| Cl | 2.4012548 | -0.8723655 | 5.3720558 |

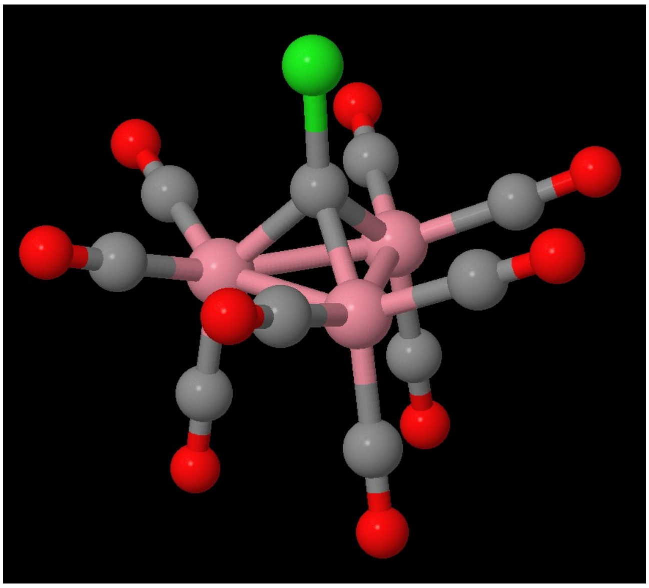

## $Co_4(CO)_{12}$

28

Atoms.

| | | | |
|---|---|---|---|
| Co | 1.8990415 | 9.8766820 | 5.7195774 |
| Co | 2.3588074 | 8.6249079 | 7.7665571 |
| Co | 1.9850356 | 11.0382917 | 7.8684180 |
| Co | 4.0715416 | 10.1631042 | 6.8651957 |
| C | 2.5722433 | 10.0512273 | 4.1181368 |
| C | 2.3120882 | 8.0215264 | 5.9483528 |
| C | 3.5258265 | 7.4637269 | 8.3468055 |
| C | 2.4376568 | 9.8097919 | 9.2681214 |
| C | 0.8889354 | 7.8074049 | 8.2629145 |
| C | 2.7577748 | 12.4422856 | 8.5606102 |
| C | 1.7335939 | 11.7461863 | 6.1078972 |
| O | 3.0195247 | 10.1659333 | 3.0773400 |
| O | 2.4529537 | 7.0546688 | 5.3264533 |
| O | 4.2927476 | 6.7102936 | 8.7219456 |
| O | 2.6433376 | 9.7934974 | 10.4077310 |
| O | 3.2698037 | 13.3545633 | 9.0101725 |
| C | 0.2163384 | 9.6315025 | 5.2916816 |
| C | 0.3432527 | 11.3247040 | 8.4135387 |
| O | -0.0660878 | 7.2800405 | 8.5866389 |
| O | 1.5684867 | 12.7573472 | 5.5678802 |
| O | -0.8770351 | 9.4682237 | 5.0217532 |
| O | -0.7248661 | 11.5025506 | 8.7634323 |
| C | 4.9805571 | 8.9726824 | 5.9294310 |
| C | 4.5677980 | 11.6478308 | 6.0477515 |
| C | 5.0743274 | 10.2513626 | 8.3162290 |
| O | 4.9179493 | 12.5965476 | 5.5254406 |
| O | 5.5922865 | 8.2218129 | 5.3315177 |
| O | 5.7453706 | 10.3105937 | 9.2336959 |

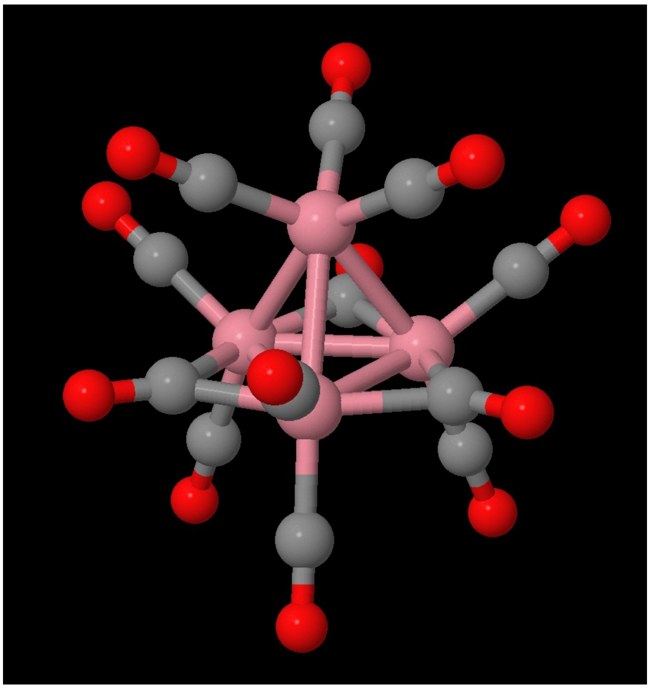

## $Co(CO)_2C_5H_5$

15
Atoms.

| | | | |
|---|---|---|---|
| Co | 0.1548470 | -0.1061959 | 0.0905793 |
| C | 1.3310553 | 0.6555247 | 1.0724957 |
| C | 1.3441910 | -0.9512616 | -0.8019594 |
| C | -1.4820215 | 1.1788463 | 0.0044591 |
| C | -1.4720363 | 0.3577179 | -1.1314547 |
| C | -1.5429854 | 0.3290122 | 1.1621982 |
| C | -1.5151619 | -1.0033195 | -0.6801392 |
| C | -1.6047349 | -1.0170692 | 0.7361590 |
| H | -1.4204867 | 2.2533741 | 0.0180745 |
| H | -1.4033468 | 0.6799984 | -2.1559000 |
| H | -1.5413369 | 0.6691624 | 2.1841271 |
| H | -1.4917937 | -1.8713822 | -1.3174633 |
| H | -1.6642884 | -1.8875578 | 1.3652773 |
| O | 2.1183967 | 1.1677716 | 1.7322669 |
| O | 2.1399424 | -1.5214212 | -1.4016005 |

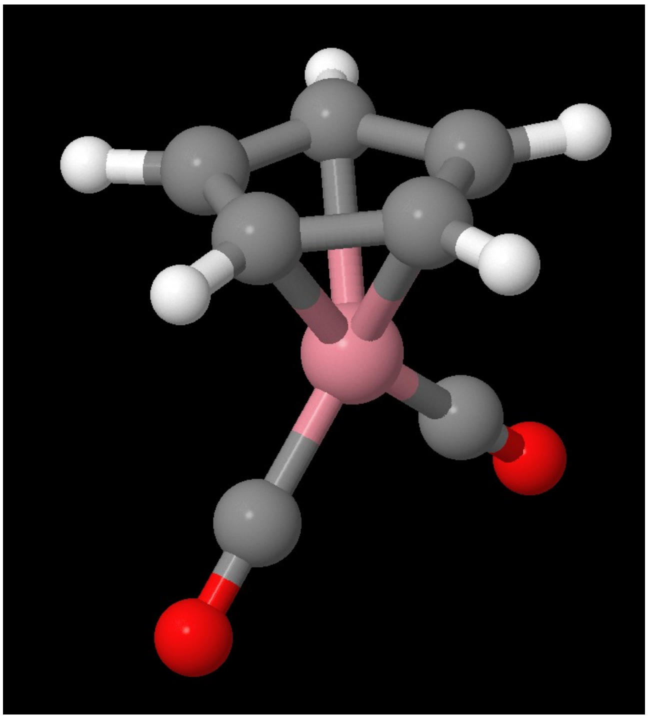

**$Co(CO)_3NO$**

```
9
Atoms.
C       -0.0193053    0.0223158   -0.5077887
Co       1.6743848   -0.2286964   -0.0336756
C        2.1958961    1.4060162    0.4256560
C        2.4823726   -0.4659308   -1.5977834
N        1.9377506   -1.3950871    1.0798232
O        2.5383846    2.4457406    0.7393021
O       -1.1101809    0.1682405   -0.8000390
O        2.1265547   -2.2167095    1.8621464
O        3.0101627   -0.6360393   -2.5924011
```

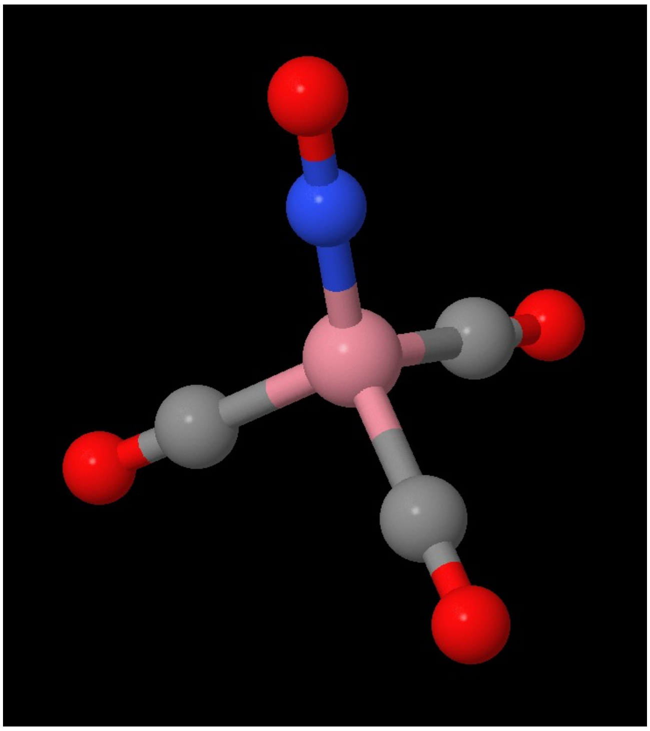

**$Co(CO)_4H$**

```
10
Atoms.
Co        -0.2063715      -0.0033284      -0.0009560
H          1.2614142      -0.0042588      -0.0013311
C         -1.9798339       0.0011358      -0.0007298
O         -3.1164682       0.0054232      -0.0009007
C          0.0624391      -1.7450418       0.0817173
O          0.2873524      -2.8602817       0.1339416
C          0.0664411       0.7931734      -1.5511006
O          0.2948643       1.3026888      -2.5437016
C          0.0683185       0.9410043       1.4633038
O          0.2982840       1.5476653       2.3993371
```

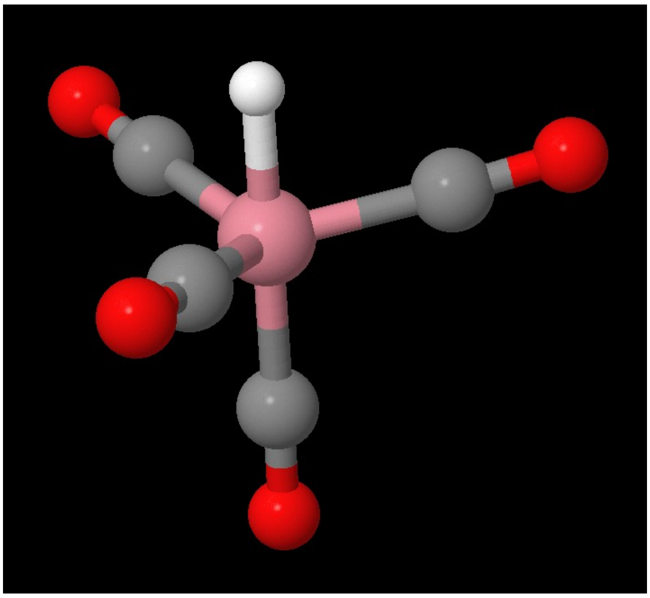

**$Cr(C_5H_5)(CO)_2NO$**

17

Atoms.

| | | | |
|---|---|---|---|
| Cr | -0.0465611 | 0.1710308 | -0.1763406 |
| N | 1.5523507 | -0.2745089 | 0.0543343 |
| C | 0.3176454 | 1.9682053 | -0.3014551 |
| C | -0.4199623 | 0.3293184 | 1.6166721 |
| O | 2.6576107 | -0.6255162 | 0.1726819 |
| O | 0.5436879 | 3.0879467 | -0.4109673 |
| O | -0.6664684 | 0.4016121 | 2.7350598 |
| C | -0.8083314 | -1.6916954 | -1.0791038 |
| C | -1.8542290 | -1.0692374 | -0.3662129 |
| C | -2.1013719 | 0.1978476 | -0.9585126 |
| C | -1.1963350 | 0.3496463 | -2.0429546 |
| C | -0.4008976 | -0.8127177 | -2.1177183 |
| H | -0.3771205 | -2.6537044 | -0.8593158 |
| H | -1.1279024 | 1.2054203 | -2.6928312 |
| H | -2.3730784 | -1.4808518 | 0.4827256 |
| H | -2.8435122 | 0.9119632 | -0.6453943 |
| H | 0.3931157 | -0.9918890 | -2.8228773 |

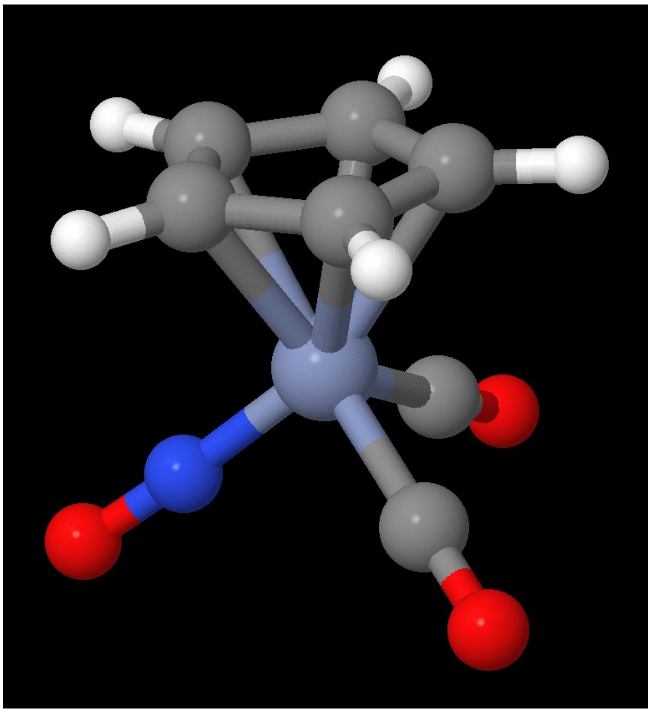

**$Cr(C_5H_5)(CO)_2NS$**

```
17
Atoms.
Cr        -0.0560891      0.1811795     -0.1771681
N          1.5434936     -0.2805696      0.0707671
C          0.3011705      1.9826169     -0.3339286
C         -0.4590550      0.3816393      1.6092638
S          2.9913221     -0.7837077      0.2303874
O          0.5192002      3.1009249     -0.4599700
O         -0.7231174      0.4817587      2.7203756
C         -0.7873708     -1.6809506     -1.1078557
C         -1.8360212     -1.1039469     -0.3588741
C         -2.1394238      0.1625240     -0.9268724
C         -1.2622544      0.3623614     -2.0231914
C         -0.4312779     -0.7735569     -2.1375182
H         -0.3132653     -2.6269587     -0.9077136
H         -1.2347150      1.2313411     -2.6586689
H         -2.3252886     -1.5483057      0.4911374
H         -2.8966394      0.8474769     -0.5852431
H          0.3579716     -0.9109568     -2.8571374
```

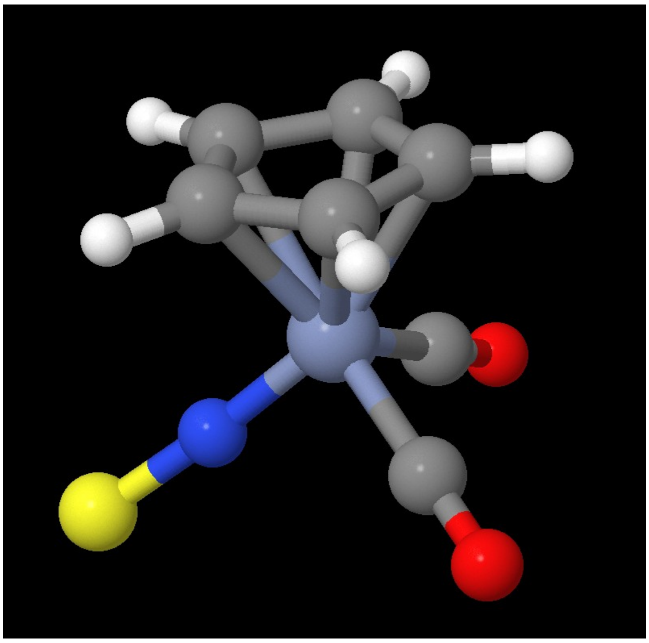

## $Cr(C_5H_5)(NO)_2Cl$

```
16
Atoms.
Cr        -0.1193918     0.2089799    -0.1525788
Cl         2.0884554    -0.1785140    -0.5276991
N         -0.0844944     1.8701764     0.0539166
N         -0.1773575    -0.0595084     1.4990244
O         -0.2830833     2.9987193     0.2159526
O         -0.4364942    -0.2026299     2.6177917
C         -1.0251091    -1.6786128    -0.8534799
C         -2.0439836    -0.7960067    -0.3922743
C         -2.0277609     0.3515423    -1.2059539
C         -1.0003988     0.1860068    -2.1797789
C         -0.3967697    -1.0670831    -1.9576823
H         -0.7519326    -2.6175120    -0.4033282
H         -0.7068017     0.9142015    -2.9164982
H         -2.6874005    -0.9580688     0.4570649
H         -2.6566400     1.2188759    -1.0882329
H          0.4770227    -1.4366263    -2.4620336
```

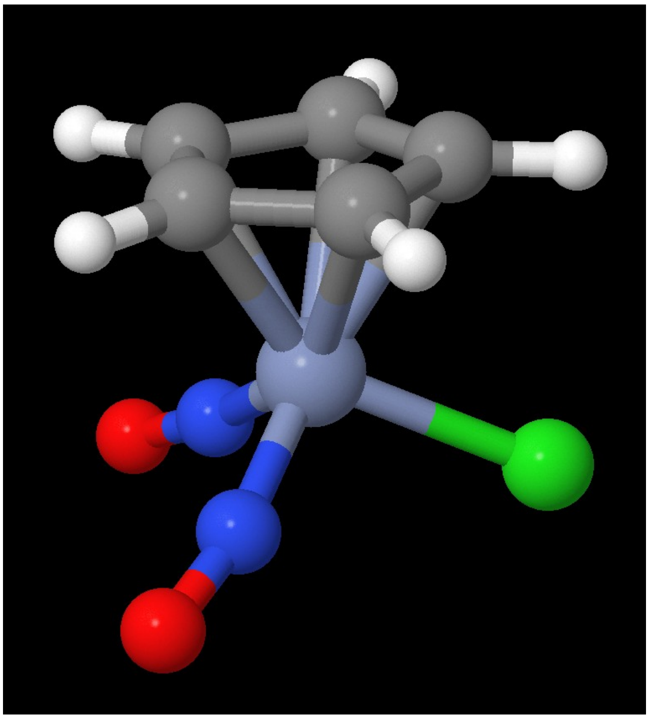

**$Cr(C_5H_5)(NO)_2NO_2$**

18

Atoms.

| | | | |
|---|---|---|---|
| Cr | -0.2160255 | 0.2163410 | 0.0592533 |
| N | 1.7493886 | -0.1466160 | -0.1711852 |
| N | -0.1109008 | 1.8830560 | 0.3136833 |
| N | -0.3239653 | -0.1661432 | 1.7011162 |
| O | -0.1708087 | 3.0273183 | 0.4774704 |
| O | -0.5286972 | -0.4209284 | 2.8114864 |
| C | -0.9841566 | -1.6755878 | -0.8049087 |
| C | -2.0692477 | -0.8137104 | -0.4777843 |
| C | -1.9517850 | 0.3517035 | -1.2644382 |
| C | -0.7935210 | 0.2153347 | -2.0812742 |
| C | -0.2131867 | -1.0394223 | -1.8004640 |
| H | -0.7727423 | -2.6312688 | -0.3561357 |
| H | -0.4121524 | 0.9478600 | -2.7722016 |
| H | -2.8306061 | -1.0088238 | 0.2585831 |
| H | -2.6074882 | 1.2056309 | -1.2361816 |
| H | 0.7000105 | -1.4186168 | -2.2258685 |
| O | 2.2155345 | -1.1608922 | 0.3314417 |
| O | 2.4044198 | 0.6175452 | -0.8679925 |

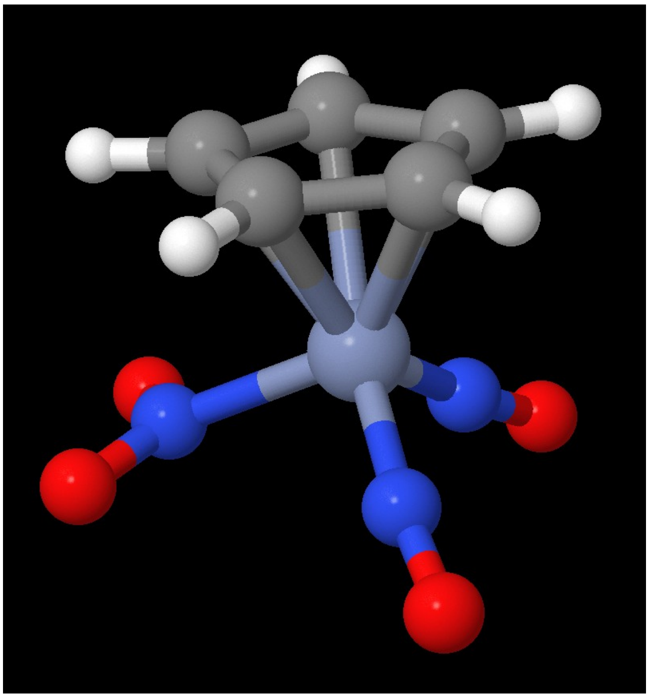

**$Cr(C_6H_5CH_3)(CO)_3$**

22

Atoms.

| | | | |
|---|---|---|---|
| Cr | 1.6322724 | -0.0022444 | 0.0200214 |
| C | -0.0138733 | 1.4544370 | -0.0725349 |
| C | -0.0049078 | 0.6898114 | -1.2474029 |
| C | -0.0624513 | -0.7196100 | -1.1911508 |
| C | -0.0890376 | -1.3446521 | 0.0618759 |
| C | -0.0980388 | -0.5808878 | 1.2507221 |
| C | -0.0335907 | 0.8229752 | 1.1969042 |
| H | 0.0846525 | 2.5282905 | -0.1300128 |
| H | 0.0973869 | 1.1823961 | -2.2028617 |
| H | 0.0020795 | -1.3053214 | -2.0947749 |
| H | -0.0514859 | -2.4220434 | 0.1240540 |
| H | -0.0651700 | -1.0803946 | 2.2074318 |
| C | 0.0248547 | 1.6380012 | 2.4486516 |
| C | 2.7180329 | 0.9982934 | 1.0623658 |
| C | 2.6800754 | -1.4200504 | 0.4345917 |
| C | 2.7735856 | 0.3340352 | -1.3448123 |
| O | 3.4051264 | 1.6346548 | 1.7305861 |
| O | 3.3589765 | -2.3081725 | 0.7027034 |
| O | 3.5150585 | 0.5483305 | -2.1968786 |
| H | 0.6084708 | 2.5435758 | 2.2969204 |
| H | -0.9804379 | 1.9297052 | 2.7553284 |
| H | 0.4794411 | 1.0734502 | 3.2598020 |

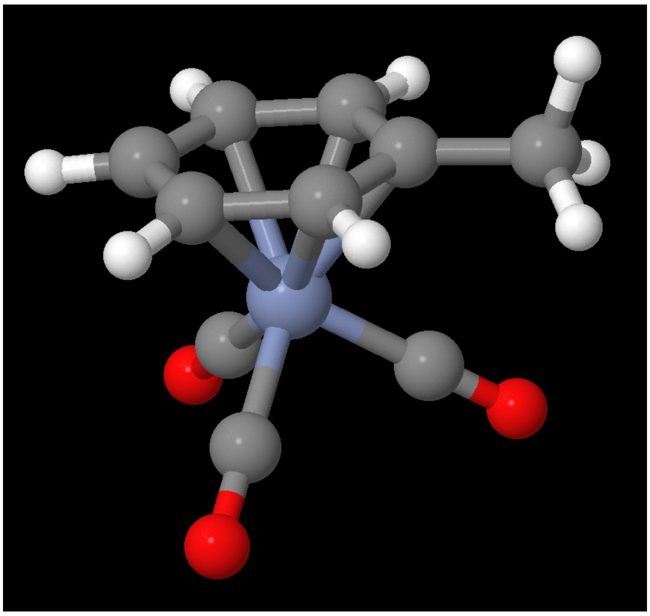

## $Cr(C_6H_5Cl)(CO)_3$

19
Atoms.

| | | | |
|---|---|---|---|
| Cr | 1.5202186 | 0.0052065 | -0.0214982 |
| C | -0.0454994 | 1.5522613 | -0.2199068 |
| C | 0.0526622 | 0.8724909 | -1.4438672 |
| C | -0.0525759 | -0.5322765 | -1.4406935 |
| C | -0.2957604 | -1.2381812 | -0.2509478 |
| C | -0.3555319 | -0.5311755 | 0.9632488 |
| C | -0.2533137 | 0.8717633 | 0.9920254 |
| Cl | 0.0695329 | 3.2722048 | -0.2040270 |
| H | 0.2422202 | 1.4200432 | -2.3526414 |
| H | 0.0688424 | -1.0692248 | -2.3694554 |
| H | -0.3531235 | -2.3148667 | -0.2578860 |
| H | -0.4685395 | -1.0684021 | 1.8929051 |
| H | -0.2933753 | 1.4197727 | 1.9192448 |
| C | 2.7329382 | 1.3655301 | 0.1786625 |
| C | 2.3580090 | -0.8763320 | 1.3442868 |
| C | 2.6852819 | -0.7948970 | -1.1824888 |
| O | 3.4916765 | 2.2194822 | 0.3044018 |
| O | 2.8709642 | -1.4368772 | 2.2087335 |
| O | 3.4059234 | -1.3042719 | -1.9212465 |

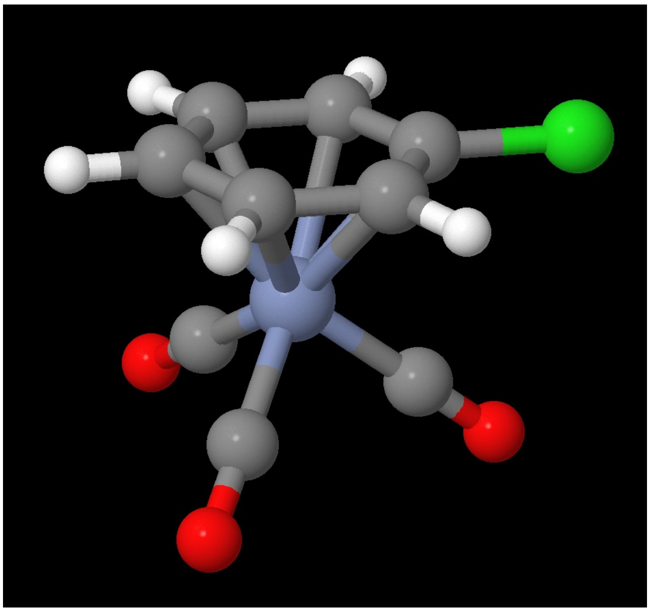

## $Cr(C_6H_6)(CO)_2CS$

19
Atoms.

| | | | |
|---|---|---|---|
| Cr | 1.5009545 | -0.0062352 | -0.0484342 |
| C | -0.0730052 | 1.5768548 | 0.0118383 |
| C | 0.0355783 | 1.0728011 | -1.3067081 |
| C | -0.0962823 | -0.2997934 | -1.5428826 |
| C | -0.3248738 | -1.1840007 | -0.4647591 |
| C | -0.4061774 | -0.6855801 | 0.8393922 |
| C | -0.2941005 | 0.7058825 | 1.0774909 |
| H | 0.0748541 | 2.6301852 | 0.1988501 |
| H | 0.2613552 | 1.7468138 | -2.1183090 |
| H | 0.0371385 | -0.6897596 | -2.5393053 |
| H | -0.3641876 | -2.2475067 | -0.6382855 |
| H | -0.5201920 | -1.3603299 | 1.6738176 |
| H | -0.3173765 | 1.0837329 | 2.0888103 |
| C | 2.7498121 | 1.2746028 | -0.3304981 |
| C | 2.3510329 | -0.3861746 | 1.5048770 |
| C | 2.6455851 | -1.1521159 | -0.8334419 |
| O | 3.5402395 | 2.0899610 | -0.4970218 |
| O | 2.8904271 | -0.6163974 | 2.4915452 |
| S | 3.6926581 | -2.1242808 | -1.4836659 |

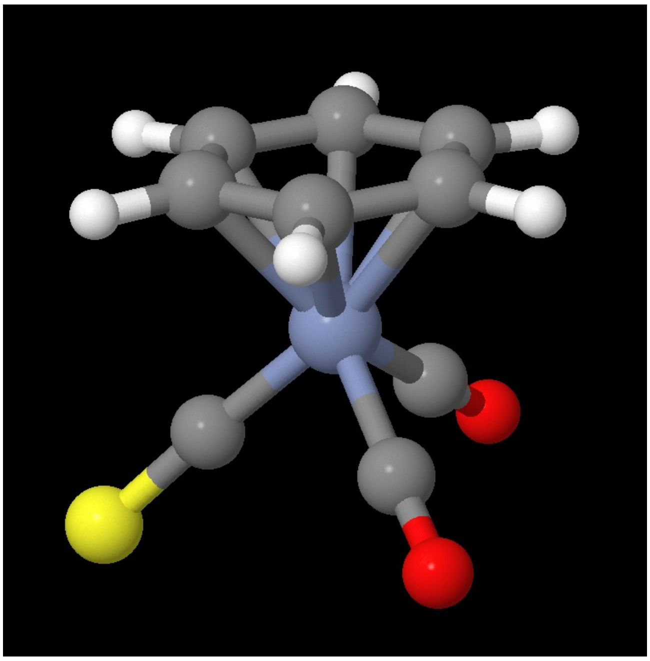

## $Cr(C_6H_6)(CO)_3$

19

Atoms.

| | | | |
|---|---|---|---|
| Cr | 1.4898753 | 0.0190700 | -0.0272413 |
| C | -0.0619170 | 1.5639144 | -0.0015909 |
| C | 0.0542491 | 1.0578979 | -1.3195970 |
| C | -0.0482146 | -0.3175841 | -1.5494802 |
| C | -0.2771690 | -1.2034097 | -0.4680941 |
| C | -0.3910030 | -0.7012964 | 0.8319574 |
| C | -0.2873284 | 0.6916534 | 1.0677654 |
| H | 0.0880184 | 2.6166532 | 0.1830867 |
| H | 0.2925319 | 1.7259746 | -2.1328293 |
| H | 0.1097948 | -0.7124616 | -2.5414521 |
| H | -0.2915502 | -2.2687191 | -0.6396952 |
| H | -0.4943479 | -1.3796325 | 1.6650515 |
| H | -0.3108701 | 1.0690790 | 2.0784492 |
| C | 2.7597699 | 1.2773598 | -0.3180593 |
| C | 2.3620758 | -0.3813548 | 1.5088964 |
| C | 2.5884962 | -1.1587676 | -0.8564312 |
| O | 3.5762164 | 2.0658418 | -0.4983542 |
| O | 2.9285204 | -0.6347687 | 2.4762948 |
| O | 3.2962917 | -1.9007896 | -1.3753667 |

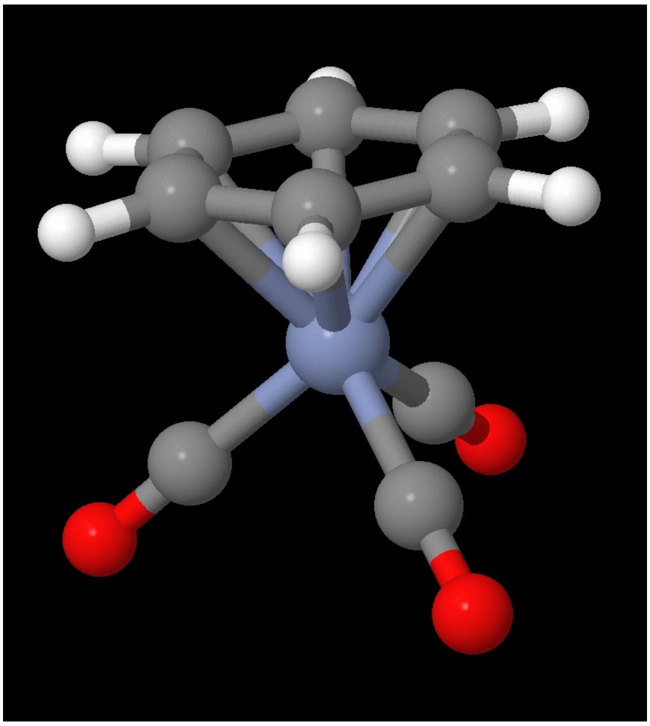

**$Cr(CO)_5C(OCH_3)CH_3$**

21
Atoms.

| | | | |
|---|---|---|---|
| Cr | 0.1122550 | -0.0350117 | 0.1769121 |
| C | 1.9695627 | 0.0691912 | 0.1292949 |
| C | 0.0055737 | 1.8204992 | 0.0883291 |
| C | 0.1559293 | -1.8956469 | 0.1952776 |
| C | -1.7445296 | -0.1120224 | 0.1003257 |
| C | 0.1493810 | -0.1011257 | -1.6753137 |
| C | 0.0197492 | 0.1146177 | 2.1736476 |
| O | 3.1042223 | 0.1512441 | 0.0168830 |
| O | 0.1520755 | -3.0375726 | 0.1462770 |
| O | -2.8821310 | -0.1481844 | 0.0154357 |
| O | 0.1815619 | -0.1478157 | -2.8160964 |
| O | -0.0701534 | 2.9567710 | 0.0129540 |
| C | -0.9428954 | 1.0156963 | 2.8811742 |
| O | 0.7526842 | -0.4606183 | 3.0907468 |
| C | 1.8461129 | -1.3444546 | 2.7987383 |
| H | 1.5427375 | -2.1075204 | 2.0920363 |
| H | 2.1058227 | -1.7885139 | 3.7530738 |
| H | 2.6804895 | -0.7711696 | 2.4089875 |
| H | -0.5199620 | 2.0250643 | 2.8567110 |
| H | -1.0885849 | 0.7357606 | 3.9229988 |
| H | -1.8947112 | 1.0709018 | 2.3605767 |

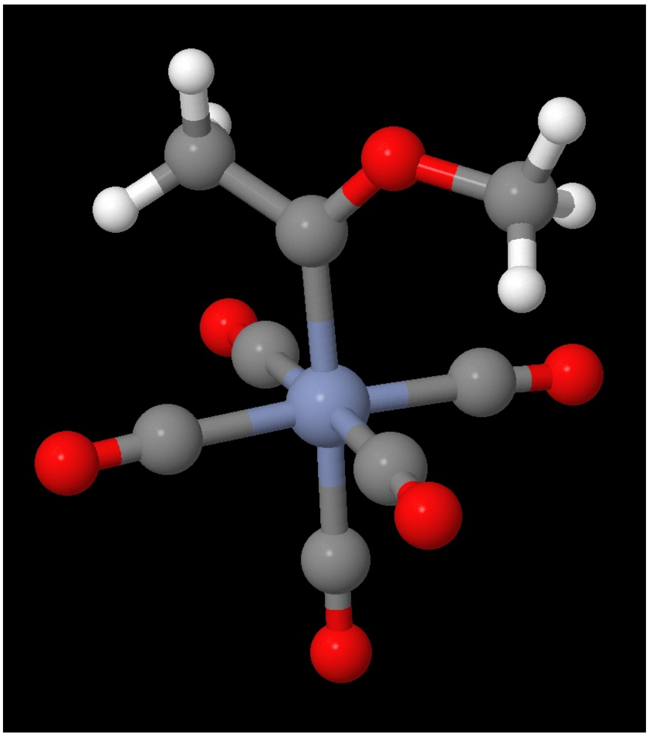

## $Cr(CO)_5CS$

13
Atoms.

| | | | |
|---|---|---|---|
| Cr | 0.0000000 | 0.0497704 | -0.0000000 |
| C | 1.8928219 | 0.0252167 | -0.0000000 |
| C | -0.0000000 | 1.9614540 | 0.0000000 |
| C | -0.0000000 | -1.8119160 | 0.0000000 |
| C | -1.8928219 | 0.0252167 | -0.0000000 |
| C | 0.0000000 | 0.0252167 | -1.8928219 |
| C | 0.0000000 | 0.0252167 | 1.8928219 |
| O | 3.0314357 | -0.0113434 | -0.0000000 |
| S | -0.0000000 | -3.3551566 | 0.0000000 |
| O | -3.0314357 | -0.0113434 | -0.0000000 |
| O | 0.0000000 | -0.0113434 | -3.0314357 |
| O | 0.0000000 | -0.0113434 | 3.0314357 |
| O | -0.0000000 | 3.1003554 | 0.0000000 |

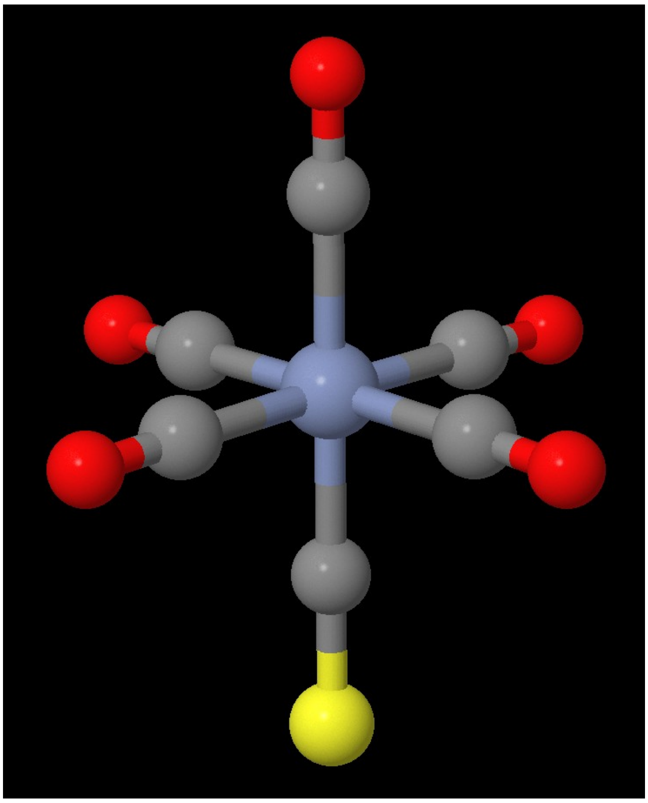

## $Cr(CO)_5PF_3$

15
Atoms.

| | | | |
|---|---|---|---|
| Cr | 0.0188224 | 0.1356592 | -0.0000000 |
| C | 1.9069296 | 0.1676573 | -0.0000002 |
| C | -0.0238942 | 2.0140969 | 0.0000000 |
| P | -0.0222954 | -2.0757959 | 0.0000000 |
| C | -1.8655671 | 0.1045425 | 0.0000001 |
| C | 0.0352024 | 0.1373864 | -1.8864177 |
| C | 0.0352027 | 0.1373862 | 1.8864176 |
| O | 3.0467163 | 0.1930040 | -0.0000003 |
| O | -3.0066746 | 0.0904858 | 0.0000002 |
| O | 0.0507959 | 0.1443163 | -3.0268539 |
| O | 0.0507965 | 0.1443160 | 3.0268539 |
| O | -0.0600660 | 3.1536716 | 0.0000000 |
| F | -0.7339377 | -2.8107591 | -1.1760878 |
| F | -0.7339397 | -2.8107589 | 1.1760868 |
| F | 1.3019188 | -2.8969081 | 0.0000013 |

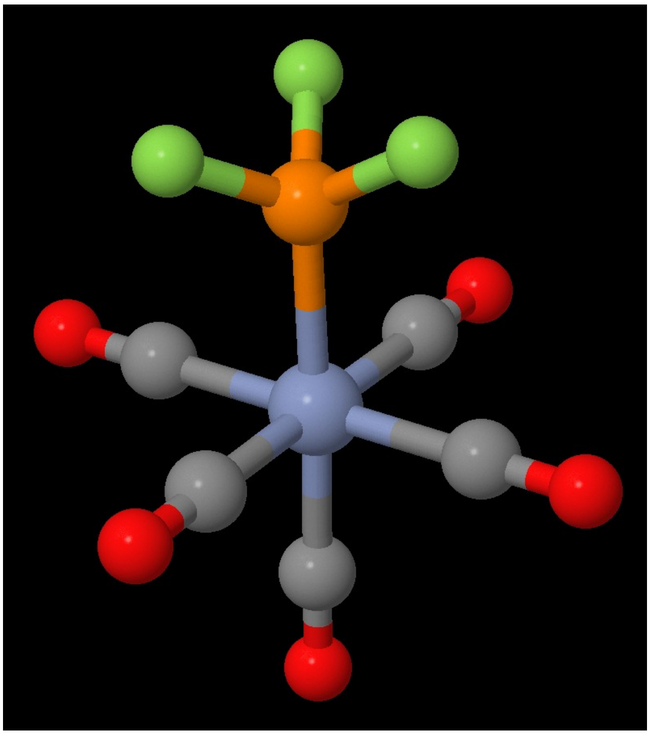

**$Cr(CO)_6$**

```
13
Atoms.
Cr      -0.0000000     0.0000000     0.0000000
C        1.8912289     0.0000000     0.0000000
C        0.0000000     1.8912289     0.0000000
C        0.0000000    -1.8912289     0.0000000
C       -1.8912289     0.0000000     0.0000000
C       -0.0000000    -0.0000000    -1.8912289
C       -0.0000000     0.0000000     1.8912289
O        3.0308617    -0.0000000    -0.0000000
O        0.0000000    -3.0308617    -0.0000000
O       -3.0308617    -0.0000000    -0.0000000
O        0.0000000    -0.0000000    -3.0308617
O        0.0000000    -0.0000000     3.0308617
O        0.0000000     3.0308617    -0.0000000
```

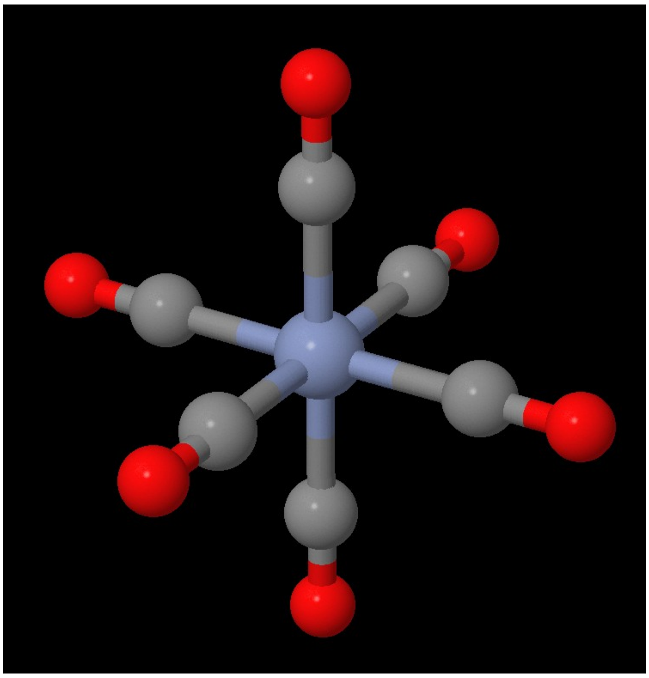

### $CrO_2Cl_2$

```
5
Atoms.
Cr        1.0203527     0.0000000    -0.0000000
Cl        2.2316364     1.7151166     0.0000000
Cl        2.2316364    -1.7151166     0.0000000
O         0.1259273    -0.0000000     1.2670195
O         0.1259273     0.0000000    -1.2670195
```

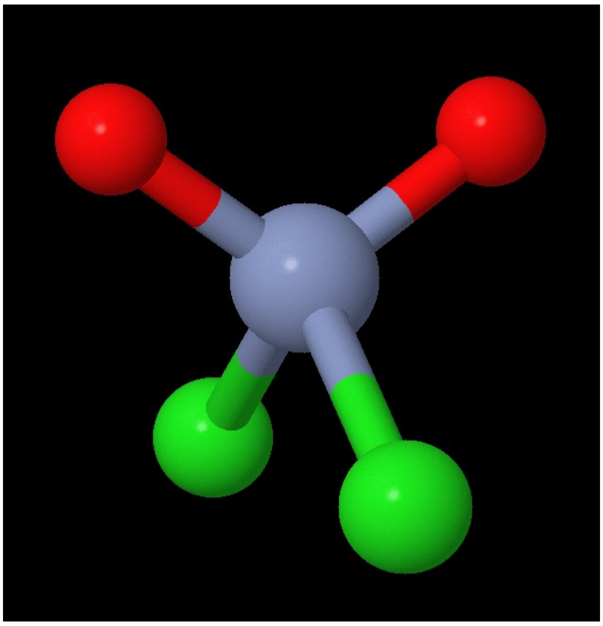

**$Fe(C_5H_5)_2$**

21

Atoms.

| | | | |
|---|---|---|---|
| Fe | -0.0014404 | 0.0000030 | 0.0053349 |
| C | 1.2109319 | -0.0000341 | -1.6082972 |
| C | 0.3753090 | -1.1510522 | -1.6100379 |
| C | -0.9778978 | -0.7114483 | -1.6133203 |
| C | -0.9779257 | 0.7114779 | -1.6133191 |
| C | 0.3752698 | 1.1510667 | -1.6100399 |
| H | 2.2873356 | 0.0000011 | -1.5736685 |
| H | 0.7085370 | -2.1747945 | -1.5786656 |
| H | -1.8487937 | -1.3446128 | -1.5869393 |
| H | -1.8487661 | 1.3445938 | -1.5869415 |
| H | 0.7085402 | 2.1748028 | -1.5786649 |
| C | 0.9772633 | 0.7114847 | 1.6220013 |
| C | -0.3759074 | 1.1510397 | 1.6214857 |
| C | -1.2114768 | 0.0000520 | 1.6215507 |
| C | -0.3759118 | -1.1511087 | 1.6214893 |
| C | 0.9773479 | -0.7115026 | 1.6220008 |
| H | 1.8481479 | 1.3445712 | 1.5927432 |
| H | -0.7091878 | 2.1748111 | 1.5912103 |
| H | -2.2879728 | -0.0000039 | 1.5903935 |
| H | -0.7091813 | -2.1747968 | 1.5912100 |
| H | 1.8481092 | -1.3445503 | 1.5927446 |

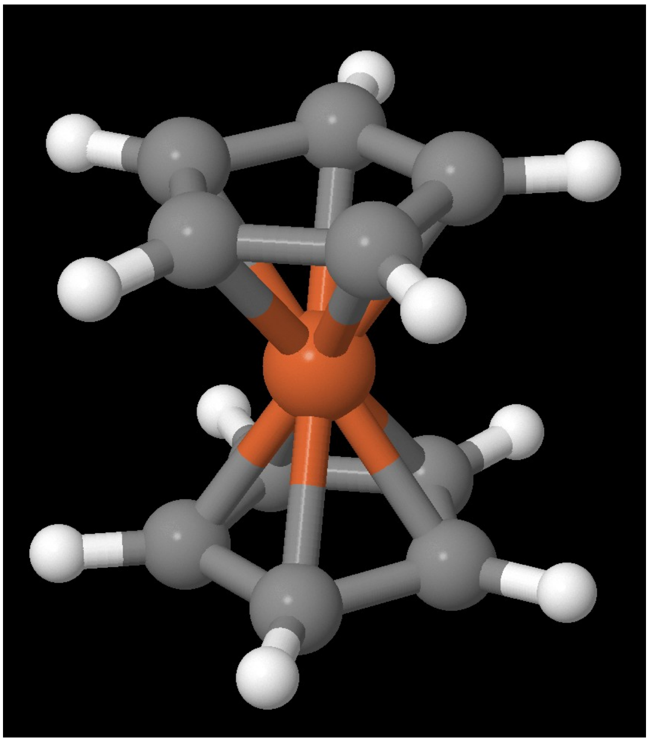

**Fe(CO)$_2$(NO)$_2$**

```
9
Atoms.
Fe      -0.0000015     0.3445392    -0.0000118
N        1.0729396     1.0081298     1.0729658
C       -0.9172726    -0.8571916     0.9173612
N       -1.0729806     1.0080330    -1.0730460
C        0.9173335    -0.8571692    -0.9173086
O        1.8500017     1.3503566     1.8499930
O       -1.4780897    -1.6735686     1.4780593
O       -1.8499851     1.3504326    -1.8499525
O        1.4780546    -1.6735619    -1.4780603
```

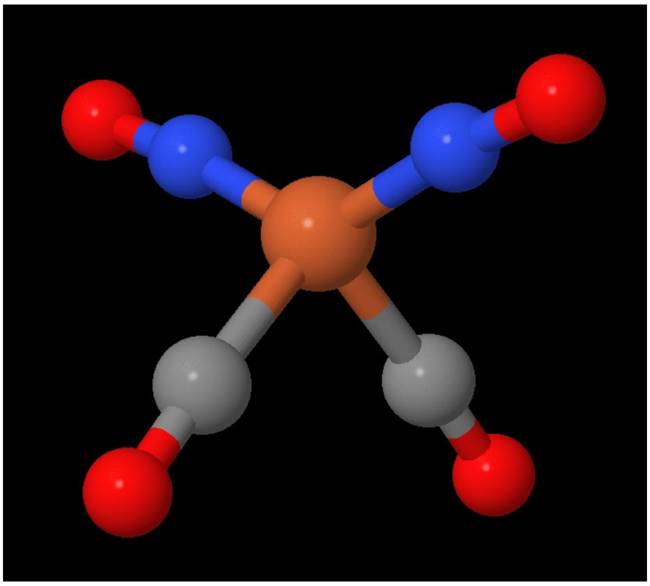

**$Fe(CO)_3C_4H_6$**

17
Atoms.

| | | | |
|---|---|---|---|
| C | 6.3266003 | 8.3252317 | 2.7471432 |
| C | 3.8999011 | 9.6070564 | 3.1019145 |
| C | 3.8996333 | 7.0428245 | 3.1022633 |
| C | 5.8551244 | 9.6726644 | 5.0864612 |
| C | 5.8550844 | 6.9772911 | 5.0864524 |
| C | 4.7544949 | 9.0282693 | 5.7085935 |
| C | 4.7545497 | 7.6217990 | 5.7086122 |
| Fe | 4.9085747 | 8.3250097 | 3.7995110 |
| O | 7.2959556 | 8.3248991 | 2.1367364 |
| O | 3.2681223 | 10.4586077 | 2.6669529 |
| O | 3.2682394 | 6.1913824 | 2.6666950 |
| H | 3.8861185 | 7.0774450 | 6.0512036 |
| H | 3.8860394 | 9.5726138 | 6.0512421 |
| H | 6.8619953 | 9.3283493 | 5.2785778 |
| H | 5.7802107 | 10.7374852 | 4.9169312 |
| H | 5.7802123 | 5.9123960 | 4.9169119 |
| H | 6.8619438 | 7.3216756 | 5.2786177 |

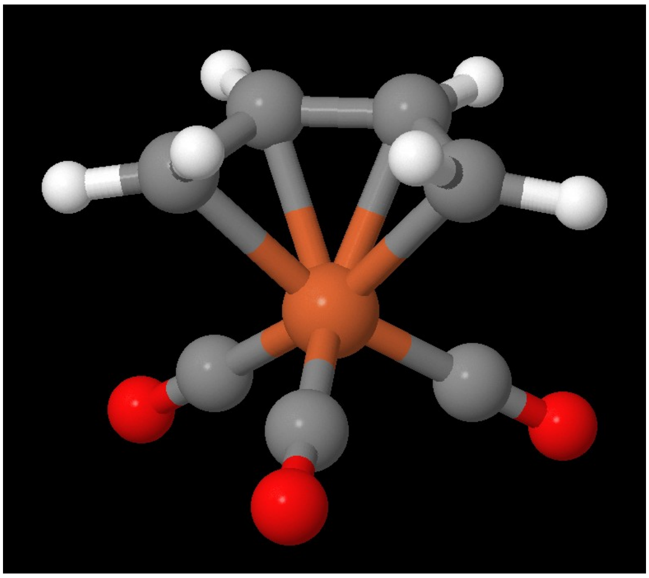

**$Fe(CO)_4C_2H_4$**

```
15
Atoms.
Fe       -0.0000022    0.0000272    0.0659505
C         1.7894444    0.0000066    0.1393406
C        -1.7894348    0.0000071    0.1393229
O         2.9277831   -0.0000026    0.2179951
O        -2.9278161   -0.0000022    0.2179336
C        -0.0000085    1.4780734   -0.9172888
C        -0.0000094   -1.4782164   -0.9173985
O        -0.0000136    2.4330673   -1.5490300
O        -0.0000161   -2.4329035   -1.5488442
C         0.0000109    0.7029895    2.0386763
C         0.0000117   -0.7030030    2.0386601
H         0.9062771    1.2455948    2.2719249
H        -0.9062548    1.2455936    2.2719364
H         0.9062807   -1.2456146    2.2719064
H        -0.9062526   -1.2456171    2.2719147
```

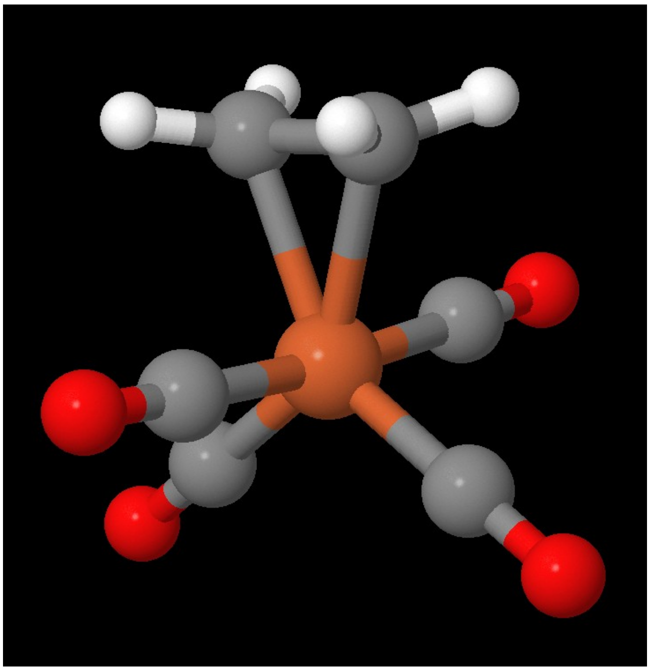

**$Fe(CO)_4H_2$**

11

Atoms.

| | | | |
|---|---|---|---|
| Fe | -0.0003703 | -0.0002204 | 0.0008637 |
| H | -0.0001018 | 0.0023518 | -1.5223484 |
| H | -0.0009474 | -0.0023485 | 1.5239877 |
| C | 1.7915722 | -0.0798343 | 0.0005364 |
| C | 0.0794659 | 1.7918169 | 0.0086007 |
| C | -1.7922892 | 0.0789498 | -0.0001368 |
| C | -0.0795629 | -1.7920406 | -0.0005139 |
| O | 2.9291128 | -0.1345335 | 0.0011459 |
| O | 0.1342972 | 2.9293104 | 0.0157687 |
| O | -2.9299136 | 0.1326378 | 0.0000548 |
| O | -0.1335529 | -2.9296494 | -0.0009087 |

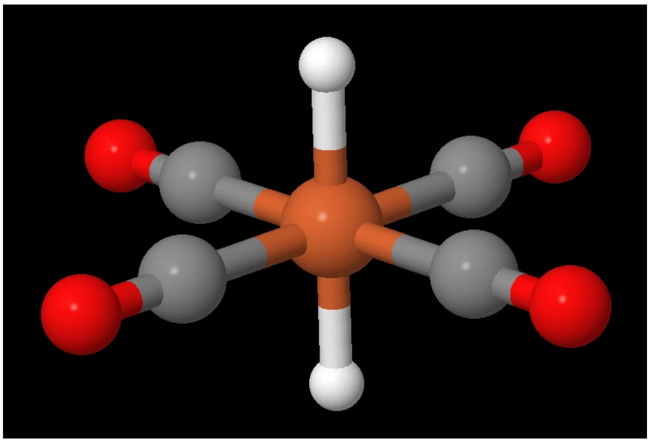

**$Fe(CO)_4P(CH_3)_3$**

22
Atoms.

| | | | |
|---|---|---|---|
| Fe | -0.0408092 | 0.0367361 | -0.1024984 |
| P | 2.1714520 | -0.0308071 | -0.0288053 |
| C | 0.1577622 | 1.7978044 | -0.2380401 |
| C | -0.0458511 | -1.7433347 | -0.0788551 |
| C | -0.8691338 | 0.1515964 | 1.4616082 |
| C | -1.0343130 | 0.0120673 | -1.5699747 |
| O | 0.3122873 | 2.9337028 | -0.3289020 |
| O | -0.0417374 | -2.8918993 | -0.0694244 |
| O | -1.4304312 | 0.2231901 | 2.4625376 |
| O | -1.7061069 | -0.0074134 | -2.5030407 |
| C | 2.8930445 | 0.7797295 | 1.4328916 |
| C | 3.0356180 | 0.7888662 | -1.4043561 |
| C | 2.9691227 | -1.6645099 | 0.0043204 |
| H | 2.5701499 | 1.8186649 | 1.4660233 |
| H | 3.9822768 | 0.7407765 | 1.4142323 |
| H | 2.5261158 | 0.2843664 | 2.3295886 |
| H | 4.1169936 | 0.7277846 | -1.2824404 |
| H | 2.7385711 | 1.8347476 | -1.4478101 |
| H | 2.7478733 | 0.3150996 | -2.3404825 |
| H | 2.6262585 | -2.2271167 | 0.8700142 |
| H | 4.0516332 | -1.5530458 | 0.0543177 |
| H | 2.7053233 | -2.2252955 | -0.8898042 |

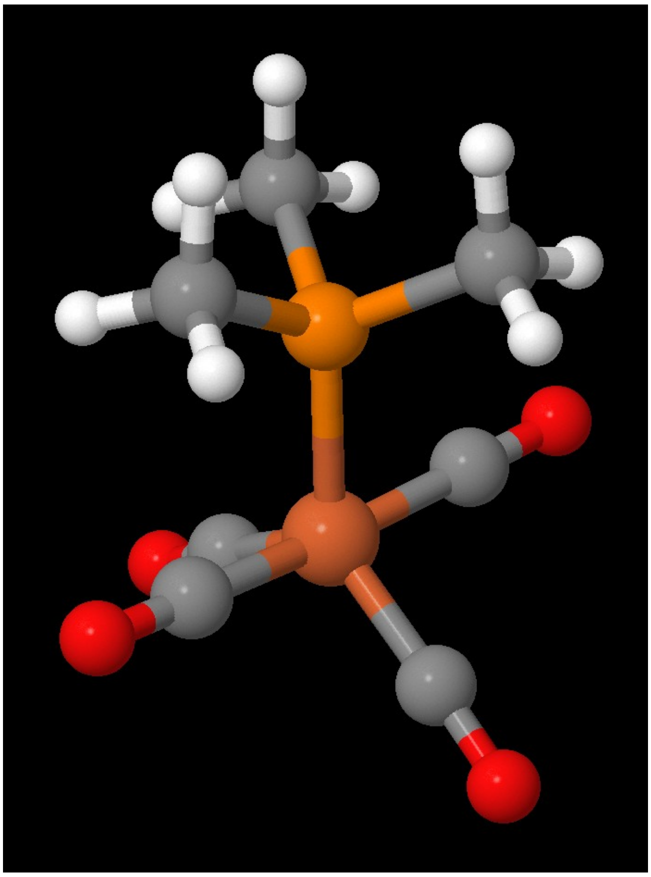

**$Fe(CO)_5$**

```
11
Atoms.
Fe      0.0064801     0.0053511    -0.0015474
C       1.8022308    -0.0039404    -0.0071946
C       0.0081266     1.8078722     0.0023630
C      -0.8585795    -0.0027087     1.5731913
C      -0.0171188    -1.7974338    -0.0321373
C      -0.9139675     0.0261317    -1.5436112
O       2.9458234    -0.0080380    -0.0059222
O       0.0052152     2.9480240    -0.0001291
O      -1.4096578    -0.0062488     2.5752463
O      -0.0398976    -2.9370625    -0.0593363
O      -1.5001748     0.0388532    -2.5256825
```

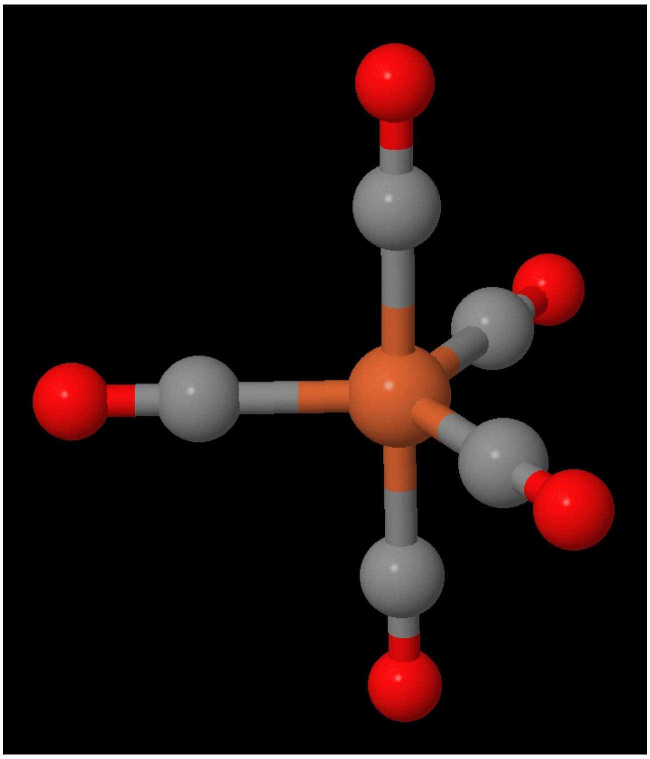

**$Mn_2(CO)_{10}$**

22

Atoms.

| | | | |
|---|---|---|---|
| Mn | -0.0182065 | 0.0079823 | -0.0031839 |
| Mn | 2.9052512 | -0.0084706 | 0.0019065 |
| C | 2.7767649 | 1.8203272 | 0.0045078 |
| C | 2.7638914 | -0.0101341 | 1.8297695 |
| C | 2.7569540 | -1.8358016 | -0.0009865 |
| C | 2.7702978 | -0.0048651 | -1.8264445 |
| C | 0.1331726 | 1.3007720 | -1.2941027 |
| C | 0.1191264 | -1.2843357 | -1.2961002 |
| C | 0.1141033 | -1.2864930 | 1.2880581 |
| C | 0.1283253 | 1.2975117 | 1.2915213 |
| C | -1.8024023 | 0.0177427 | -0.0070270 |
| C | 4.6893649 | -0.0180958 | 0.0051180 |
| O | 2.7170643 | 2.9585213 | 0.0064025 |
| O | 2.6972286 | -0.0104195 | 2.9675662 |
| O | 2.6848577 | -2.9732681 | -0.0027441 |
| O | 2.7068213 | -0.0026318 | -2.9644314 |
| O | 5.8319943 | -0.0242596 | 0.0072983 |
| O | 0.2099046 | 2.1057754 | -2.0974024 |
| O | 0.1867382 | -2.0890404 | -2.1005249 |
| O | 0.1802197 | -2.0931198 | 2.0906894 |
| O | 0.2051064 | 2.0975137 | 2.0998041 |
| O | -2.9450080 | 0.0240487 | -0.0091841 |

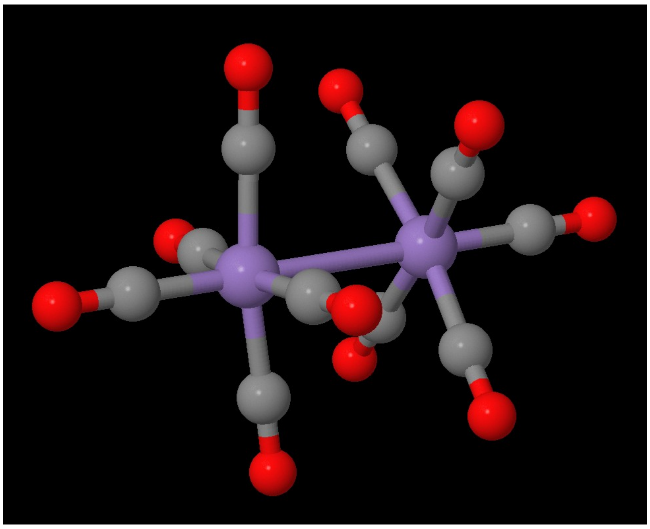

**$Mn(CO)_2(CS)C_5H_5$**

17

Atoms.

| | | | |
|---|---|---|---|
| Mn | 0.0237953 | 0.0149947 | 0.0118670 |
| C | 2.1761303 | 0.0498057 | -0.0037653 |
| C | 1.6956207 | 1.3791499 | 0.0398605 |
| C | 0.9365031 | 1.5216045 | 1.2353491 |
| C | 0.9578927 | 0.2877239 | 1.9211155 |
| C | 1.7247412 | -0.6304076 | 1.1533039 |
| H | 2.7677107 | -0.3795182 | -0.7948596 |
| H | 1.8650186 | 2.1418666 | -0.7005367 |
| H | 0.4257125 | 2.4138490 | 1.5553446 |
| H | 0.4575581 | 0.0712236 | 2.8491088 |
| H | 1.9156257 | -1.6603383 | 1.4000729 |
| C | -1.1591433 | -1.0886400 | 0.6666049 |
| C | 0.0222492 | -0.8423785 | -1.5421983 |
| C | -1.2349306 | 1.1421865 | -0.5284977 |
| S | -2.1852669 | -2.0806377 | 1.2889688 |
| O | 0.0383223 | -1.4082871 | -2.5400111 |
| O | -2.0415497 | 1.8877830 | -0.8601973 |

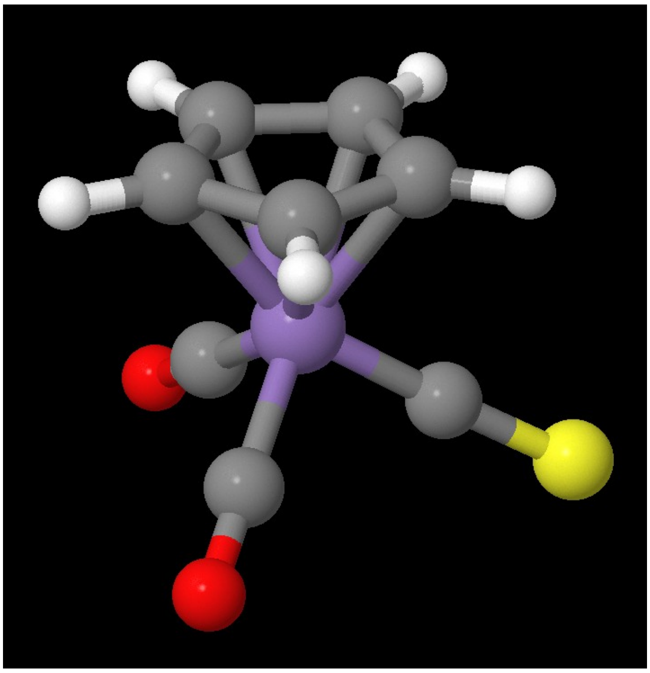

**$Mn(CO)_3C_5H_4CH_3$**

20
Atoms.

| | | | |
|---|---|---|---|
| Mn | 0.0852290 | -0.0640567 | -0.0562325 |
| C | 2.1974512 | 0.2239108 | -0.2441059 |
| C | 1.6053940 | 1.4606343 | 0.1261219 |
| C | 0.9588054 | 1.2670270 | 1.3730917 |
| C | 1.1670044 | -0.0824048 | 1.7812877 |
| C | 1.9302325 | -0.7234738 | 0.7844782 |
| H | 2.7590051 | 0.0415231 | -1.1450818 |
| C | 1.7052450 | 2.7422572 | -0.6217817 |
| H | 0.4099913 | 2.0170391 | 1.9178070 |
| H | 0.7918991 | -0.5363330 | 2.6826855 |
| H | 2.2393700 | -1.7549732 | 0.7898191 |
| C | -1.4585544 | -0.2944045 | 0.7828443 |
| C | -0.0766575 | -1.5793901 | -0.9608760 |
| C | -0.6665655 | 0.8802621 | -1.3525728 |
| O | -2.4435799 | -0.4310122 | 1.3586959 |
| O | -0.1464050 | -2.5684348 | -1.5417489 |
| O | -1.1237339 | 1.5207277 | -2.1906721 |
| H | 2.5919195 | 3.2895092 | -0.2980878 |
| H | 0.8382654 | 3.3748113 | -0.4436197 |
| H | 1.7900140 | 2.5728014 | -1.6929922 |

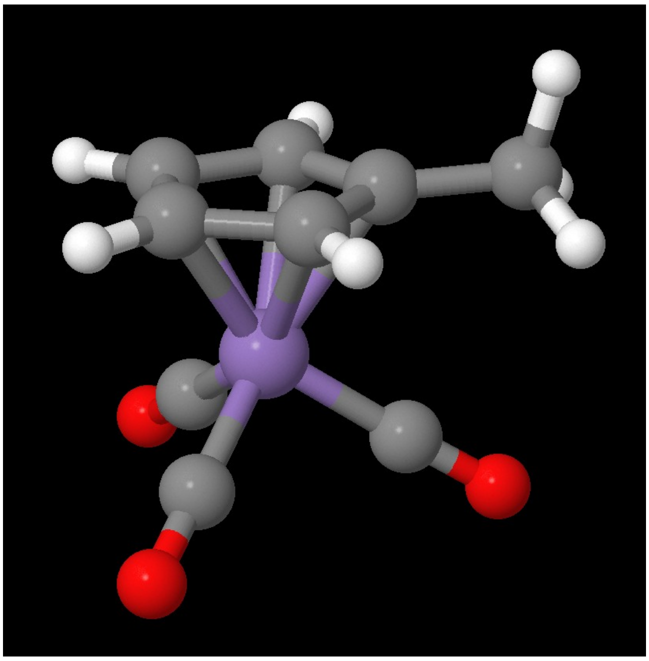

**$Mn(CO)_3C_5H_5$**

17

Atoms.

| | | | |
|---|---|---|---|
| Mn | 0.0199822 | 0.0068904 | 0.0155309 |
| C | 2.1510219 | 0.1735338 | -0.0766024 |
| C | 1.5929209 | 1.4547234 | 0.1184766 |
| C | 0.8808048 | 1.4399391 | 1.3527637 |
| C | 1.0086827 | 0.1468856 | 1.9072337 |
| C | 1.7914343 | -0.6449537 | 1.0282696 |
| H | 2.7326250 | -0.1366325 | -0.9281272 |
| H | 1.6793602 | 2.2920087 | -0.5526494 |
| H | 0.3377865 | 2.2645733 | 1.7814781 |
| H | 0.5668925 | -0.1878022 | 2.8306442 |
| H | 2.0637238 | -1.6761107 | 1.1717572 |
| C | -1.2902043 | -0.9174562 | 0.7706916 |
| C | 0.0298079 | -1.0494829 | -1.4070803 |
| C | -1.1088732 | 1.1474803 | -0.7348329 |
| O | -2.1223189 | -1.5185997 | 1.2861418 |
| O | 0.0694935 | -1.7367471 | -2.3267443 |
| O | -1.8184499 | 1.9152304 | -1.2111808 |

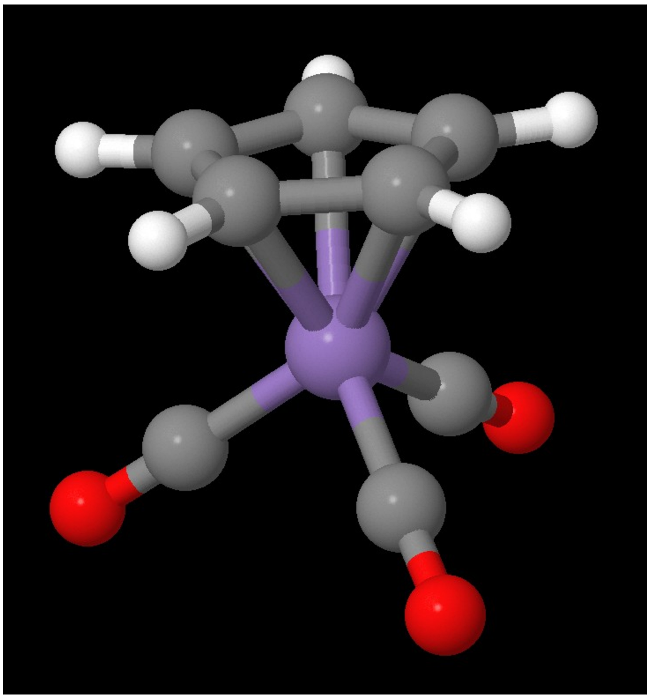

**$Mn(CO)_3C_5Me_5$**

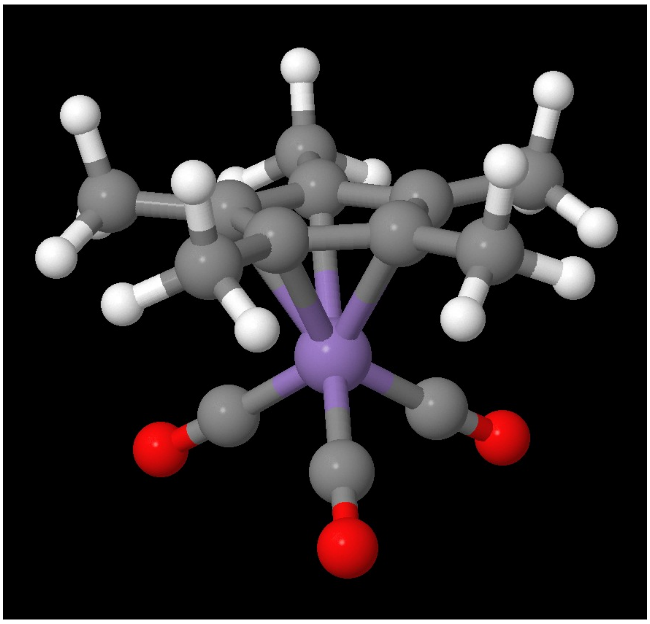

| | | | |
|---|---|---|---|
| 32 | | | |
| Atoms. | | | |
| Mn | 0.0362069 | 0.0110779 | 0.0083427 |
| C | 2.1715003 | 0.1037668 | -0.0400769 |
| C | 1.6478145 | 1.4198591 | 0.0839552 |
| C | 0.8889472 | 1.4903509 | 1.2918159 |
| C | 0.9678938 | 0.2106711 | 1.9275683 |
| C | 1.7501345 | -0.6458717 | 1.1086241 |
| C | 3.0857808 | -0.3856533 | -1.1074249 |
| C | 1.9144254 | 2.5545106 | -0.8410772 |
| C | 0.2357096 | 2.7058582 | 1.8494338 |
| C | 0.4019399 | -0.1326758 | 3.2602343 |
| C | 2.1549163 | -2.0418607 | 1.4275620 |
| C | -1.5212054 | -0.2443870 | 0.8096499 |
| C | -0.0322999 | -1.5061924 | -0.8985235 |
| C | -0.6926731 | 0.9576712 | -1.2979264 |
| O | -2.5134810 | -0.3915839 | 1.3752438 |
| O | -0.0124561 | -2.5042040 | -1.4732624 |
| O | -1.1358976 | 1.6058972 | -2.1401383 |
| H | 2.8156468 | 3.0876623 | -0.5303270 |
| H | 1.0943992 | 3.2689370 | -0.8497497 |
| H | 2.0669200 | 2.2136380 | -1.8627797 |
| H | 0.9283179 | 3.2629164 | 2.4857584 |
| H | -0.6328463 | 2.4506358 | 2.4531332 |
| H | -0.0984810 | 3.3764498 | 1.0606327 |
| H | -0.5041314 | 0.4311028 | 3.4708724 |
| H | 1.1248638 | 0.0963309 | 4.0464777 |
| H | 0.1577463 | -1.1901860 | 3.3322769 |
| H | 3.1075001 | -2.0503675 | 1.9630173 |
| H | 2.2793828 | -2.6397155 | 0.5269813 |
| H | 1.4183641 | -2.5388379 | 2.0548969 |
| H | 2.9403682 | -1.4458277 | -1.3050748 |
| H | 4.1293182 | -0.2454129 | -0.8144484 |
| H | 2.9305952 | 0.1484503 | -2.0421775 |

**$Mn(CO)_4NO$**

```
11
Atoms.
Mn    -0.0000398   -0.1510188    0.0058011
C      1.8253517    0.0584318   -0.0042912
C     -1.8250730    0.0614686   -0.0042391
O     -2.9508104    0.2294287   -0.0120973
O      2.9513840    0.2243729   -0.0127540
N     -0.0014422   -1.8215830    0.0858194
O     -0.0024812   -2.9747508    0.1404691
C      0.0008297    0.7346639   -1.5824362
O      0.0013436    1.2491507   -2.6026692
C      0.0006471    0.8844581    1.5010906
O      0.0010006    1.4955581    2.4665269
```

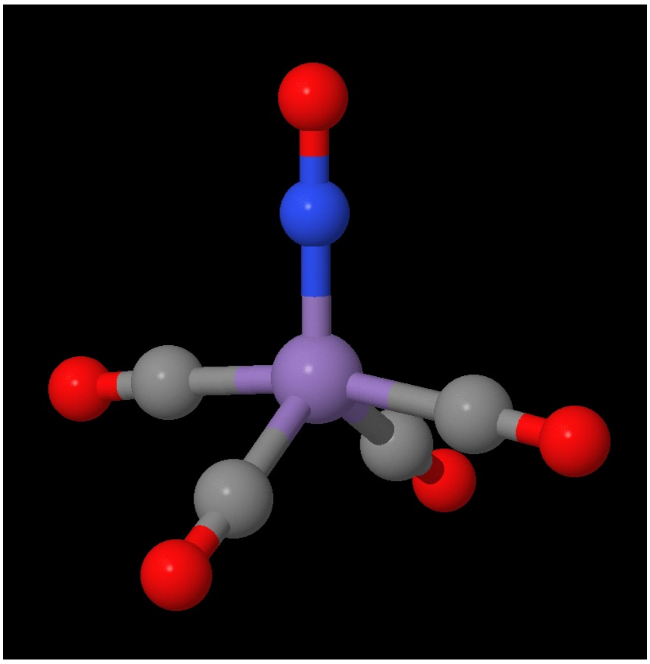

**$Mn(CO)_5Br$**

```
12
Atoms.
Mn         0.0461630      0.0041798      0.0030694
Br         2.5531934     -0.0101510     -0.0017005
C         -1.7458786      0.0137485      0.0058152
C          0.2111562      1.2301148      1.3787192
O          0.3391235      2.2200857     -1.9726895
C          0.1926587     -1.2234954     -1.3733216
C          0.2066542      1.3795036     -1.2238384
C          0.1956522     -1.3731220      1.2290786
O          0.3214196     -2.2161180      1.9763754
O          0.3469570      1.9789568      2.2187835
O         -2.8877042      0.0191493      0.0069970
O          0.3169250     -1.9734221     -2.2141882
```

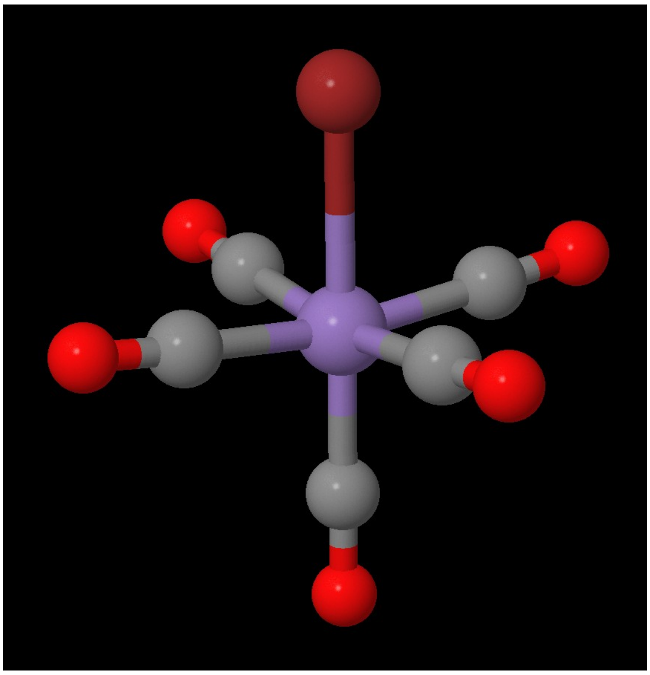

**$Mn(CO)_5CF_3$**

15
Atoms.

| | | | |
|---|---|---|---|
| Mn | 0.0628538 | -0.0101922 | -0.0006711 |
| C | 1.8876122 | 0.0107968 | 0.0009911 |
| C | -0.0731510 | 1.8272682 | 0.0019278 |
| C | -0.0363082 | -0.0324985 | -1.8398465 |
| C | -0.0256962 | -1.8487572 | -0.0045732 |
| C | -0.0403106 | -0.0391145 | 1.8382206 |
| C | -2.0233834 | 0.0546281 | -0.0006313 |
| O | -0.1038607 | -0.0587897 | -2.9718450 |
| O | -0.0855290 | -2.9815168 | -0.0072154 |
| O | -0.1787338 | 2.9566264 | 0.0034117 |
| O | 3.0270297 | 0.0342523 | 0.0019508 |
| O | -0.1104435 | -0.0697164 | 2.9699687 |
| F | -2.6291681 | -1.1588558 | 0.0129345 |
| F | -2.5414167 | 0.6943569 | -1.0838380 |
| F | -2.5392946 | 0.7167524 | 1.0702152 |

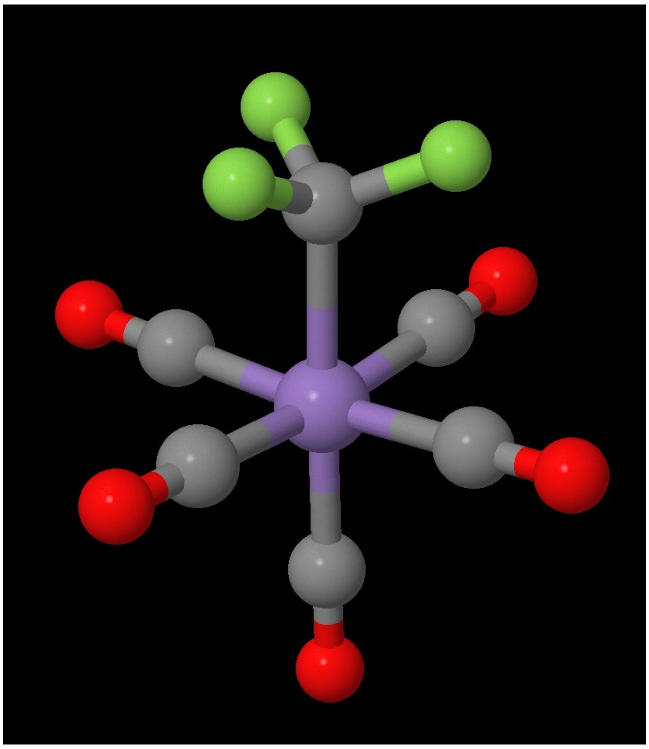

### $Mn(CO)_5CH_3$

```
15
Atoms.
Mn        0.1021946     0.0085086     0.0100513
C         1.9093767    -0.0058810    -0.0086118
C        -0.0735816     1.8272551    -0.0453019
C        -0.1161586    -0.0544792    -1.8046553
C        -0.1030691    -1.8066816     0.0878483
C        -0.0659250     0.0784927     1.8283153
C        -2.0792356     0.0118406    -0.0270154
O        -0.3210594    -0.0929869    -2.9236933
O        -0.2934751    -2.9278406     0.1394007
O        -0.2454369     2.9521894    -0.0771003
O         3.0519654    -0.0161181    -0.0255227
O        -0.2284968     0.1241586     2.9542401
H        -2.4425066    -0.8550760    -0.5720346
H        -2.4410213     0.9102618    -0.5191118
H        -2.4693207    -0.0190734     0.9860113
```

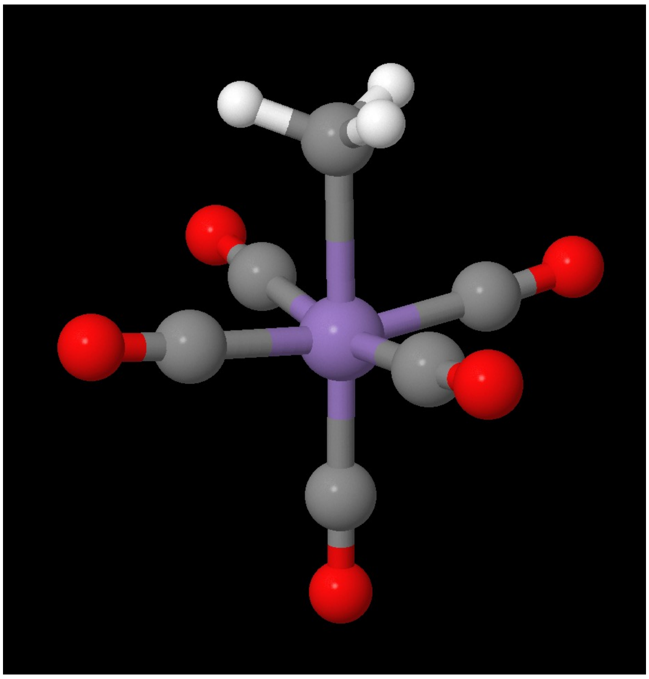

**$Mn(CO)_5Cl$**

```
12
Atoms.
Mn          0.0558477        0.0039185        0.0029217
Cl          2.4185999       -0.0088344       -0.0014183
C          -1.7382518        0.0141135        0.0060920
C           0.2192189        1.2313852        1.3803188
O           0.3588779        2.2196666       -1.9732506
C           0.2011396       -1.2252344       -1.3748450
C           0.2158392        1.3806378       -1.2256611
C           0.2048858       -1.3751430        1.2301792
O           0.3410770       -2.2170518        1.9758139
O           0.3640682        1.9789486        2.2190525
O          -2.8802320        0.0210442        0.0081865
O           0.3352495       -1.9740209       -2.2142896
```

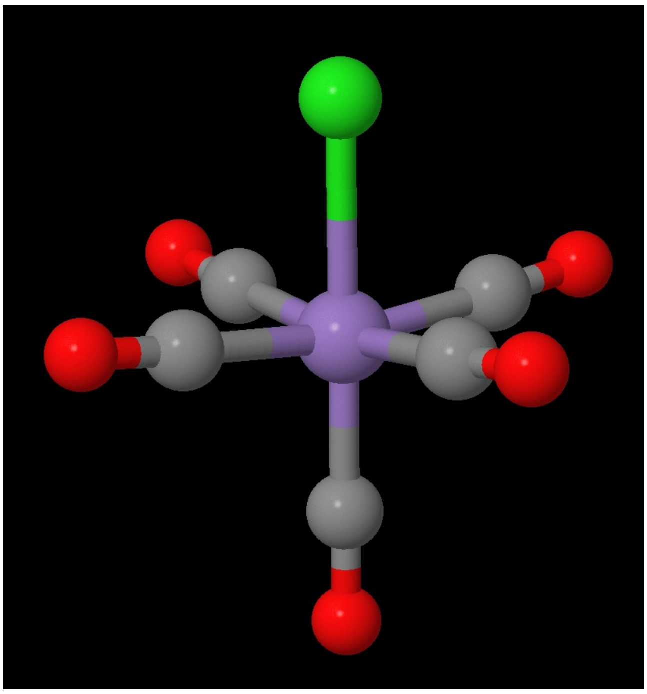

**$Mn(CO)_5COCF_3$**

17
Atoms.

| | | | |
|---|---|---|---|
| Mn | 0.0035370 | -0.0014813 | 0.0647029 |
| C | 1.8457629 | 0.0022702 | 0.0602900 |
| C | 0.0023367 | 1.8279625 | -0.0914276 |
| C | 0.0095757 | -1.8110799 | -0.2454362 |
| C | -0.1917865 | 0.0865155 | -2.0063630 |
| C | -1.8431119 | -0.0071910 | 0.1045933 |
| C | 1.1100508 | 0.1186017 | -2.8572189 |
| C | 0.0467542 | -0.0788914 | 1.8876091 |
| F | 0.8745198 | 0.1771014 | -4.1582034 |
| F | 1.8442941 | -0.9819562 | -2.6122513 |
| F | 1.8516435 | 1.1882492 | -2.5164923 |
| O | 0.0012380 | 2.9570810 | -0.2247440 |
| O | 0.0130891 | -2.9247473 | -0.4743205 |
| O | -2.9752381 | -0.0118692 | 0.1499390 |
| O | 2.9789890 | 0.0012787 | 0.1321203 |
| O | -1.2279837 | 0.1158382 | -2.6006169 |
| O | 0.0701595 | -0.1278721 | 3.0256695 |

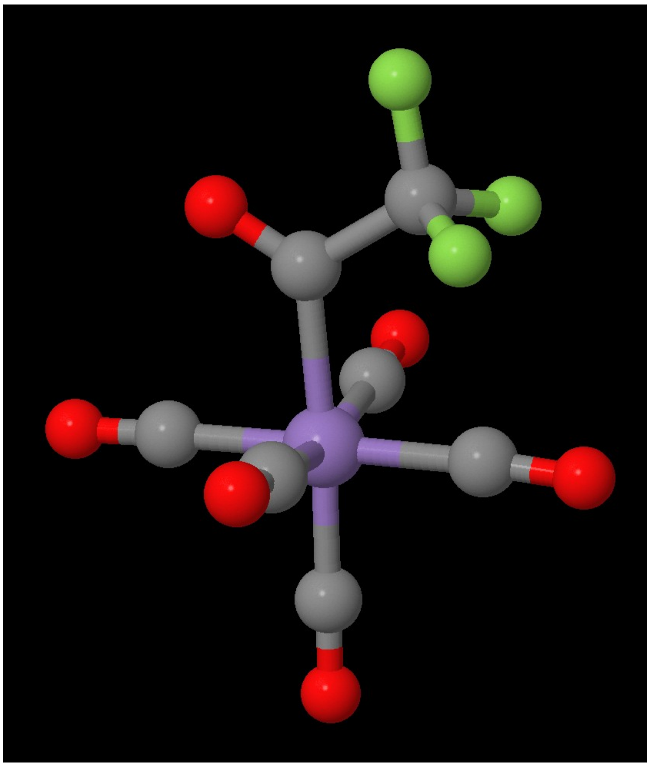

**$Mn(CO)_5COCH_3$**

17
Atoms.

| | | | |
|---|---|---|---|
| Mn | -0.0374805 | -0.0036289 | 0.0776464 |
| C | 1.7897940 | 0.0033608 | 0.0010438 |
| C | -0.0599934 | 1.8080800 | -0.1441663 |
| C | -0.0532250 | -1.7834612 | -0.3273843 |
| C | -0.2637075 | 0.1052214 | -2.0623499 |
| C | -1.8803082 | -0.0119212 | 0.1604349 |
| C | 0.9889594 | 0.1475455 | -2.8932646 |
| C | 0.0559862 | -0.0953051 | 1.8918568 |
| H | 0.7385132 | 0.2001202 | -3.9512729 |
| H | 1.5913839 | -0.7391363 | -2.6930374 |
| H | 1.5901322 | 1.0108003 | -2.6058454 |
| O | -0.0667177 | 2.9327667 | -0.3350657 |
| O | -0.0581349 | -2.8823062 | -0.6339135 |
| O | -3.0123724 | -0.0171055 | 0.2279834 |
| O | 2.9296582 | 0.0043042 | -0.0059550 |
| O | -1.3493384 | 0.1303199 | -2.5617407 |
| O | 0.1159808 | -0.1523844 | 3.0301905 |

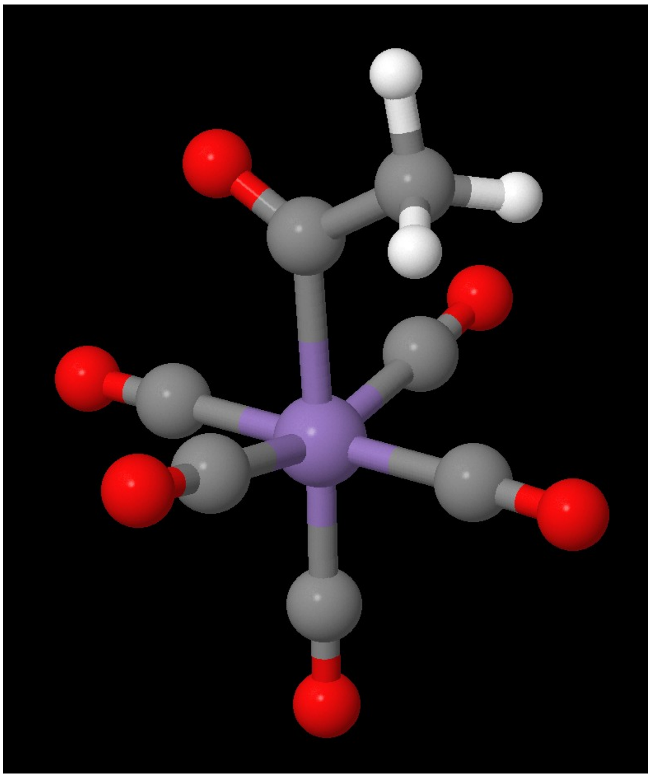

## $Mn(CO)_5H$

12
Atoms.

| | | | |
|---|---|---|---|
| Mn | 0.1170671 | 0.0002795 | -0.0003395 |
| C | 1.9402704 | -0.0033539 | 0.0001241 |
| C | -0.1055661 | 1.8129447 | -0.0007659 |
| C | -0.1092040 | 0.0003721 | -1.8126159 |
| C | -0.1127542 | -1.8115422 | -0.0000142 |
| C | -0.1103685 | 0.0010897 | 1.8116694 |
| H | -1.4445577 | 0.0033733 | -0.0007732 |
| O | -0.3114823 | 0.0003224 | -2.9324190 |
| O | -0.3169462 | -2.9310032 | 0.0002172 |
| O | -0.3054296 | 2.9331989 | -0.0009559 |
| O | 3.0812452 | -0.0056397 | 0.0002847 |
| O | -0.3133839 | 0.0017283 | 2.9313481 |

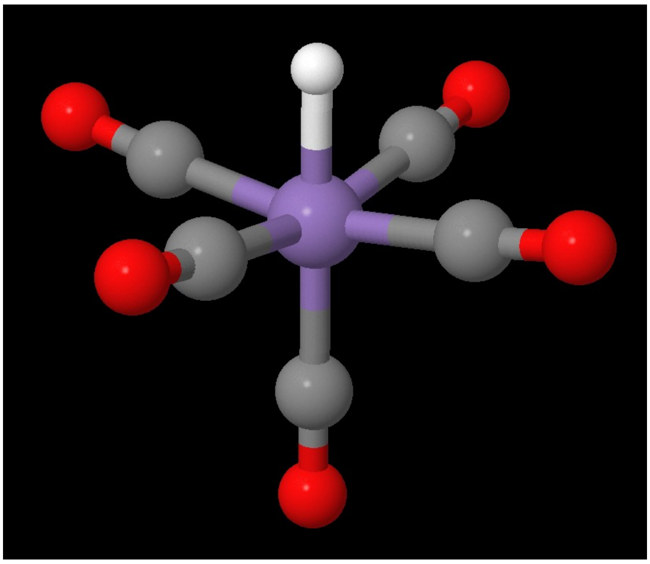

**$Mn(CO)_5I$**

12
Atoms.

| | | | |
|---|---|---|---|
| Mn | 0.0695568 | 0.0118740 | 0.0073844 |
| I | 2.7726021 | 0.0122892 | 0.0113654 |
| C | -1.7213031 | 0.0113612 | 0.0044800 |
| C | 0.2146786 | 1.2371187 | 1.3821599 |
| O | 0.3224024 | 2.2306061 | -1.9686297 |
| C | 0.2195379 | -1.2133461 | -1.3673369 |
| C | 0.2182648 | 1.3867943 | -1.2173752 |
| C | 0.2152815 | -1.3629077 | 1.2327388 |
| O | 0.3179147 | -2.2069847 | 1.9839123 |
| O | 0.3168210 | 1.9890108 | 2.2256576 |
| O | -2.8629616 | 0.0106295 | 0.0021716 |
| O | 0.3250249 | -1.9649254 | -2.2106881 |

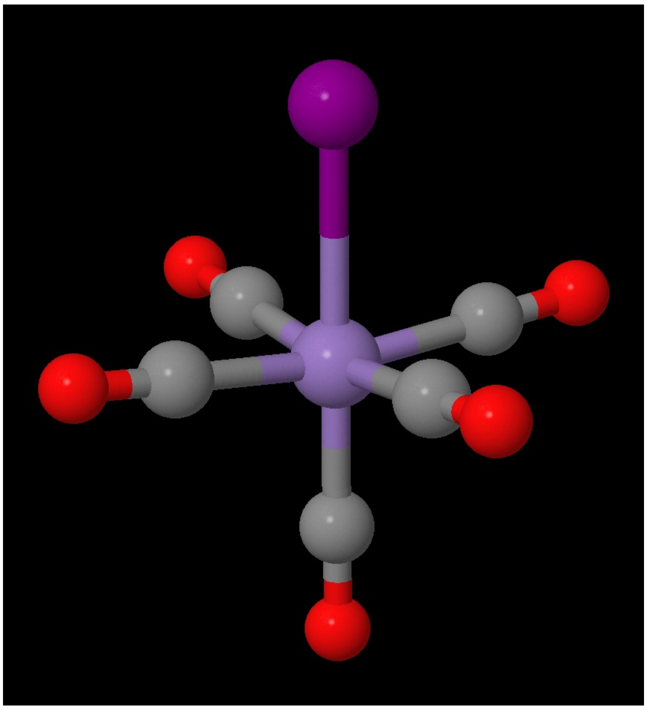

## $Mn(CO)_5SiCl_3$

15
Atoms.

| | | | |
|---|---|---|---|
| Mn | 0.0102921 | 0.0216748 | -0.0098581 |
| Si | 2.4015625 | -0.0374543 | 0.0231108 |
| C | -1.8073299 | -0.0077152 | 0.0409787 |
| C | 0.1387888 | 1.3393274 | 1.2604263 |
| O | 0.1302132 | 2.1197594 | -2.1073940 |
| C | 0.1091305 | -1.2476252 | -1.3315525 |
| C | 0.0884469 | 1.3172261 | -1.3047108 |
| C | 0.2020244 | -1.2715555 | 1.2785272 |
| O | 0.3309177 | -2.0718604 | 2.0748561 |
| O | 0.2098662 | 2.1703030 | 2.0317054 |
| O | -2.9451553 | -0.0311276 | 0.0787275 |
| O | 0.1614481 | -2.0180078 | -2.1647192 |
| Cl | 3.1875004 | 0.4079546 | 1.8749785 |
| Cl | 3.3209479 | 1.2571280 | -1.2836932 |
| Cl | 3.1613964 | -1.8986073 | -0.4282826 |

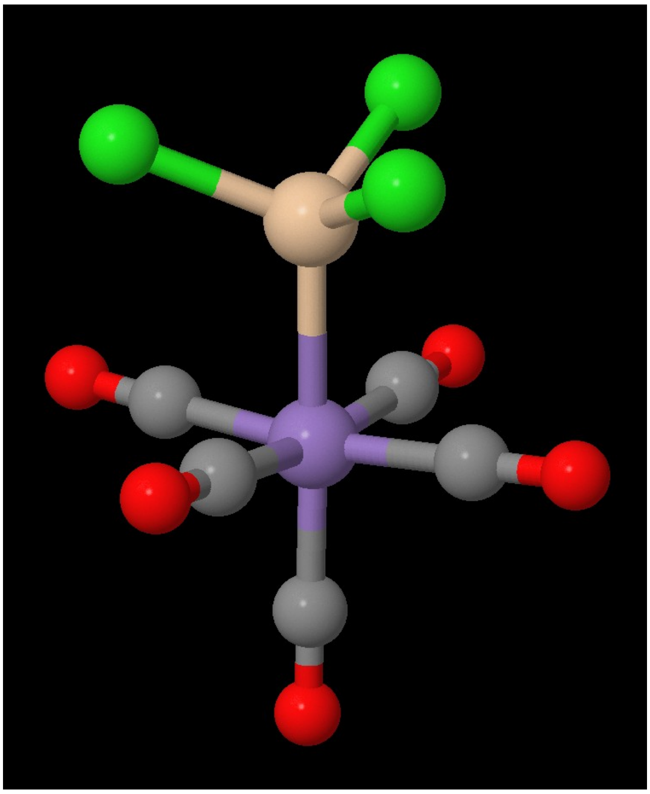

**$Mn(CO)_5SiF_3$**

```
15
Atoms.
Mn        0.0339012     0.0188983    -0.0036952
Si        2.3773527    -0.0255922     0.0114512
C        -1.7893613     0.0003962     0.0165716
C         0.1862517     1.2728035     1.3239940
O         0.2689646     2.1855404    -2.0196056
C         0.1849453    -1.2164653    -1.3481637
C         0.1683099     1.3566189    -1.2489808
C         0.2190018    -1.3139070     1.2386963
O         0.3558543    -2.1408486     2.0072764
O         0.2974254     2.0525410     2.1432259
O        -2.9274937    -0.0152654     0.0333853
O         0.2948369    -1.9772561    -2.1857583
F         3.0086011     0.4561882     1.3850802
F         3.0586290     0.8779466    -1.0996981
F         2.9628311    -1.4821785    -0.2206792
```

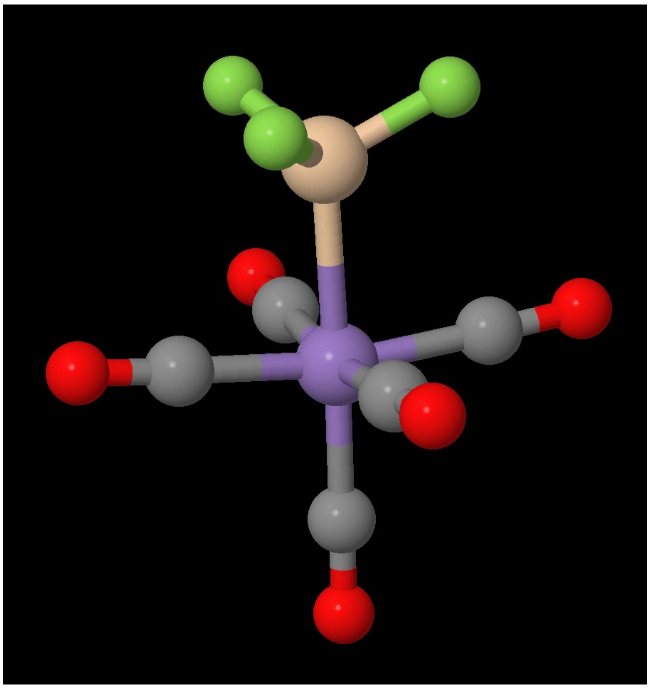

**$Mn(NO)_3CO$**

9

Atoms.

| | | | |
|---|---|---|---|
| Mn | 0.0186727 | -0.1246226 | 0.0992925 |
| N | 1.1024471 | 0.8181237 | 0.9572859 |
| N | -1.0976378 | -0.9064899 | 1.0698972 |
| C | -0.9616541 | 1.0616605 | -0.9006409 |
| N | 0.7517768 | -1.1334445 | -1.0159737 |
| O | 1.8729466 | 1.4210265 | 1.5740371 |
| O | 1.2836261 | -1.8592598 | -1.7424934 |
| O | -1.8248963 | -1.4789144 | 1.7634103 |
| O | -1.5703312 | 1.7975705 | -1.5203851 |

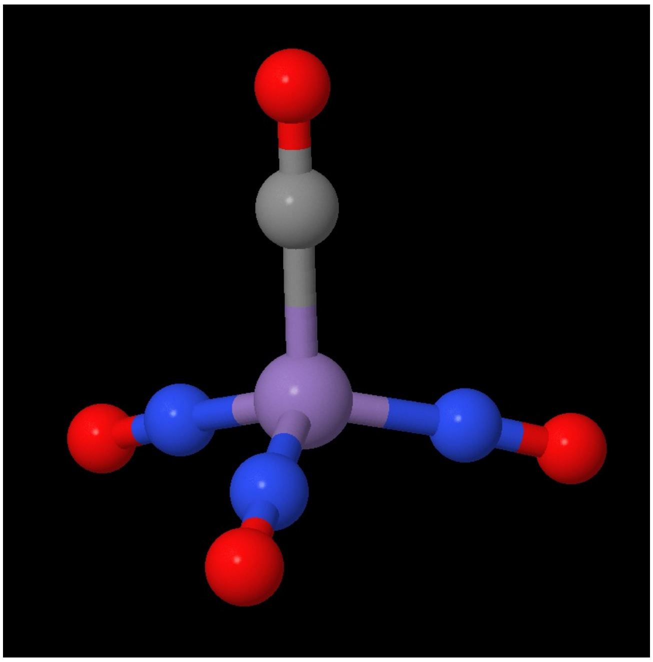

## $Mn(NO)_3P(CH_3)_3$

20
Atoms.

| | | | |
|---|---|---|---|
| Mn | 0.2773452 | -0.4114834 | 0.3398594 |
| N | 1.2118464 | 0.6617356 | 1.2024150 |
| N | -0.8678974 | -1.2301520 | 1.2272559 |
| P | -0.9539159 | 0.9289687 | -0.9290954 |
| N | 1.0957049 | -1.3268023 | -0.7834403 |
| O | 1.8882630 | 1.3800225 | 1.8301086 |
| O | 1.6919429 | -1.9925979 | -1.5375587 |
| O | -1.6374241 | -1.8288799 | 1.8728536 |
| C | -2.1399171 | 0.0813564 | -2.0108624 |
| C | -0.0127367 | 1.9787518 | -2.0729280 |
| C | -1.9840560 | 2.1136171 | -0.0171074 |
| H | 0.6746524 | 2.6025263 | -1.5043452 |
| H | -0.6736927 | 2.6130682 | -2.6647642 |
| H | 0.5737690 | 1.3469780 | -2.7376743 |
| H | -2.5660832 | 2.7385792 | -0.6954525 |
| H | -1.3446201 | 2.7444665 | 0.5978268 |
| H | -2.6579484 | 1.5694379 | 0.6421608 |
| H | -2.7093397 | 0.7921941 | -2.6108059 |
| H | -2.8232859 | -0.5066949 | -1.4007549 |
| H | -1.6023267 | -0.5991519 | -2.6687410 |

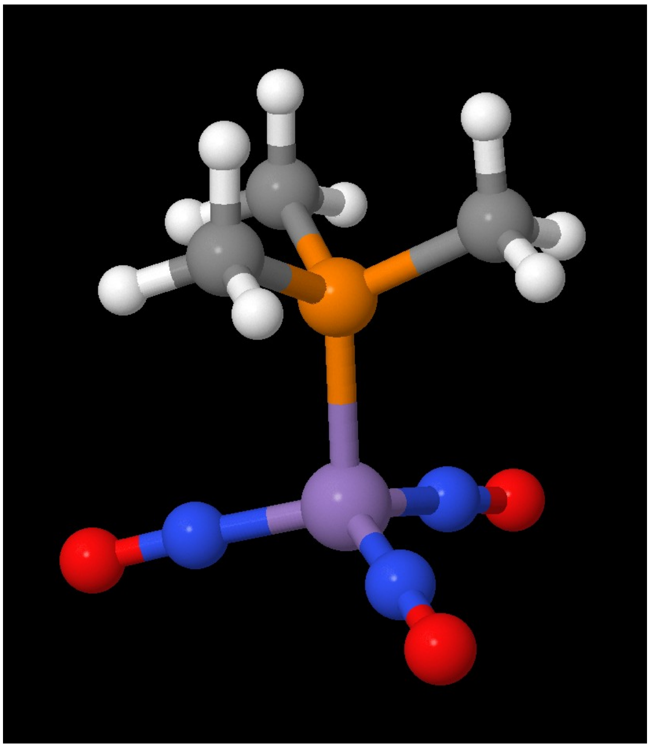

**$MnO_3Cl$**

| | | | |
|---|---|---|---|
| 5 | | | |
| Atoms. | | | |
| Mn | -0.0766778 | 0.0434510 | 0.0519714 |
| O | 0.8428397 | 0.9088783 | 0.9630144 |
| O | -0.9564256 | -0.9172678 | 0.9049202 |
| O | -0.9623889 | 0.9446318 | -0.8579149 |
| Cl | 1.1459527 | -1.1200433 | -1.1814911 |

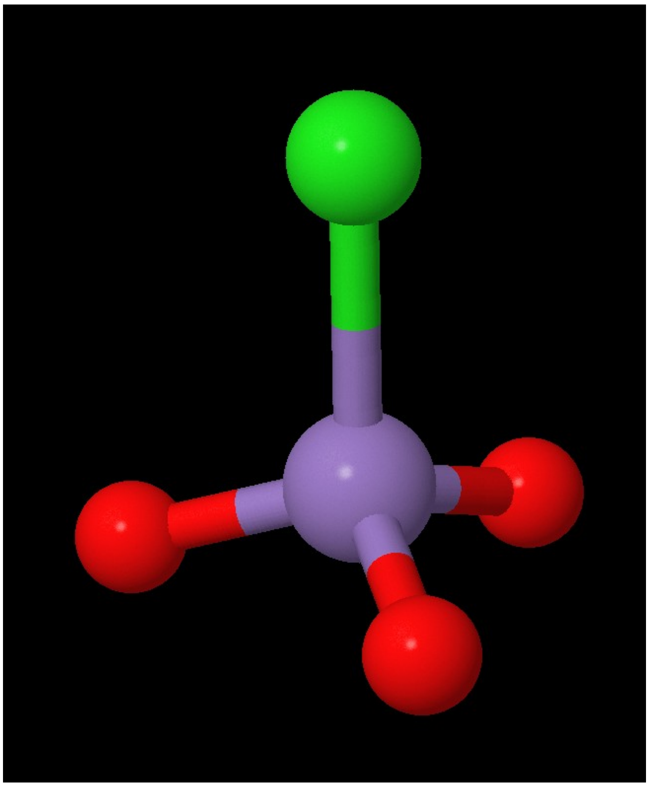

**$TiBr_4$**

```
5
Atoms.
Br          2.8141845        8.4431847        8.4438153
Ti          4.1582983        9.7872985        7.0997019
Br          5.4614917       11.1715978        8.4432979
Br          2.8147026       11.0904921        5.7154025
Br          5.5425979        8.4437028        5.7965084
```

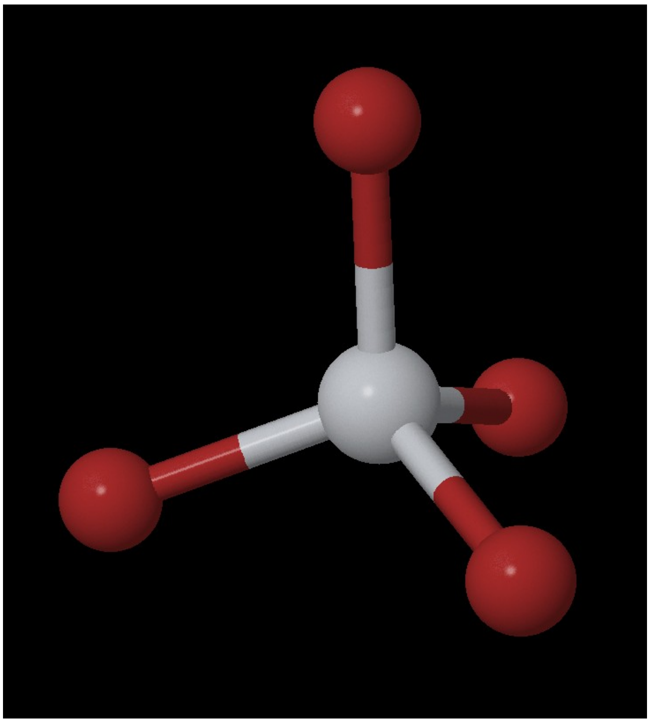

## $TiCl_4$

5
Atoms.

| | | | |
|---|---|---|---|
| Ti | 0.0003697 | -0.0006179 | 0.0005547 |
| Cl | -2.1454656 | -0.2758823 | -0.0321712 |
| Cl | 0.8451138 | -1.1005774 | 1.6616222 |
| Cl | 0.4524538 | 2.1034689 | 0.2233094 |
| Cl | 0.8475283 | -0.7264913 | -1.8533151 |

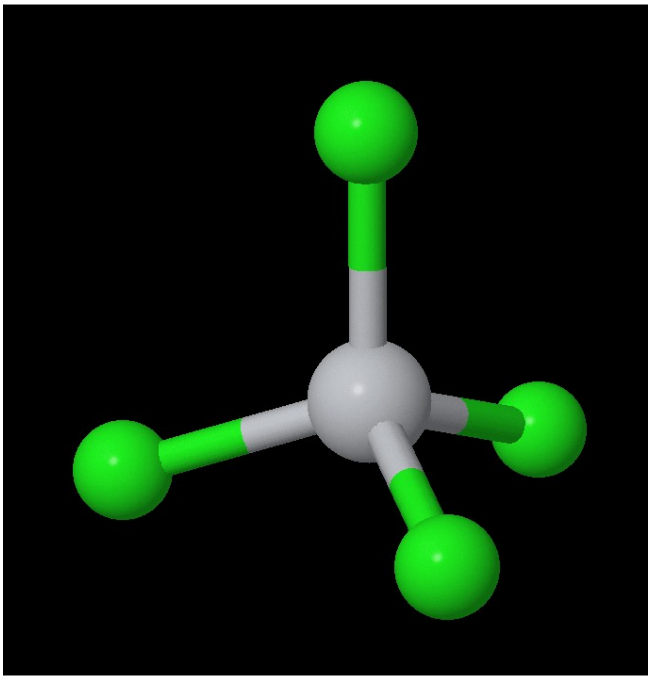

**$TiF_4$**

```
5
Atoms.
Ti        -0.0000997       -0.0003391        0.0003376
F         -1.7379343       -0.2234911       -0.0257990
F          0.6845507       -0.8913955        1.3450362
F          0.3666079        1.7036321        0.1808126
F          0.6868755       -0.5885064       -1.5003874
```

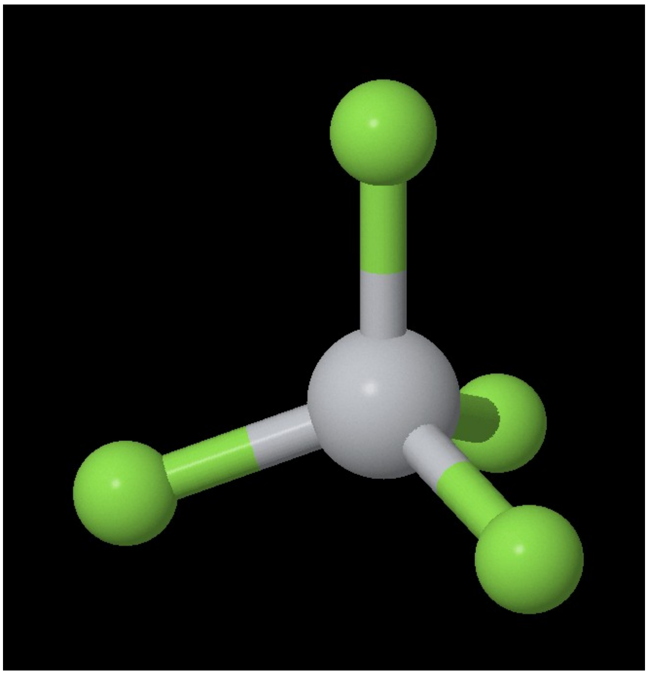

## $TiI_4$

```
5
Atoms.
I     2.6936334     8.3226338    8.5643663
Ti    4.1579809     9.7869807    7.1000195
I     5.5779883    11.2953218    8.5626500
I     2.6953506    11.2069889    5.5916786
I     5.6663217     8.3243508    5.6800116
```

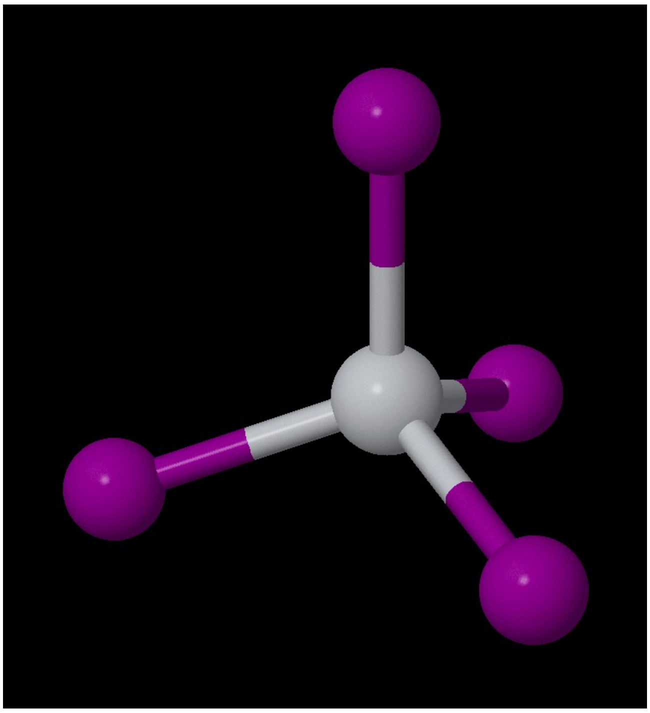

**$Ti(NO_3)_4$**

| | | | |
|---|---|---|---|
| 17 | | | |
| Atoms. | | | |
| N | -3.6071822 | -10.0673345 | 3.7347578 |
| O | -1.4863482 | -6.7635873 | 1.1043554 |
| O | 0.4952791 | -12.2272452 | 4.7315887 |
| O | -0.9077627 | -10.6385993 | 5.2590559 |
| O | -1.3190931 | -7.9657547 | 5.6732076 |
| O | -0.6892549 | -8.5705813 | 2.0237182 |
| N | -0.0995475 | -7.6078556 | 5.5429433 |
| O | 0.4232185 | -8.1259722 | 4.4790505 |
| N | -1.4176951 | -7.5213523 | 2.0038216 |
| Ti | -1.3004120 | -9.1104653 | 3.9376780 |
| O | -2.6414276 | -10.2724738 | 2.8983697 |
| O | 0.0385641 | -10.5941416 | 3.3643703 |
| N | -0.0761849 | -11.2320580 | 4.4653891 |
| O | -2.0778506 | -7.3954340 | 3.1093307 |
| O | -4.6871997 | -10.5240526 | 3.6208453 |
| O | -3.2296232 | -9.3080918 | 4.6902014 |
| O | 0.4798142 | -6.9006925 | 6.2860906 |

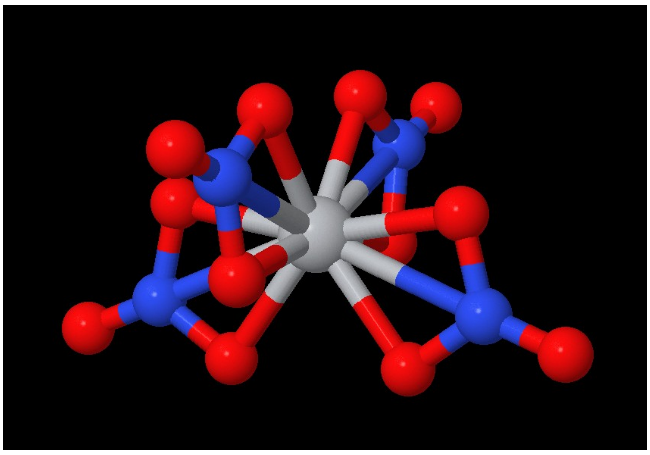

**$V(CO)_3C_7H_7$**

21
Atoms.

| | | | |
|---|---|---|---|
| V | 0.2562410 | 0.0458609 | -0.1059659 |
| C | 2.0239604 | 0.2564649 | 0.6418512 |
| C | 0.6687369 | 1.6833651 | -1.0427530 |
| C | -0.2297420 | -0.9387462 | 1.8583246 |
| C | -0.6303828 | 0.4115232 | 1.9446742 |
| C | -1.3615662 | 1.1587579 | 1.0175919 |
| C | -1.8815125 | 0.7449054 | -0.2276498 |
| H | -1.4485938 | 2.2153971 | 1.2297729 |
| H | -0.2256527 | 0.9647760 | 2.7807844 |
| H | -2.3086246 | 1.5327804 | -0.8331957 |
| H | 0.4411411 | -1.2703357 | 2.6393063 |
| C | 1.1925535 | -0.7915856 | -1.5702088 |
| C | -0.4873461 | -1.8757935 | 0.8501300 |
| C | -1.1698100 | -1.6681025 | -0.3613031 |
| C | -1.8204483 | -0.5145047 | -0.8352185 |
| H | -1.1243747 | -2.4910830 | -1.0620115 |
| H | -2.2066005 | -0.5724522 | -1.8431480 |
| H | 0.0065786 | -2.8314597 | 0.9549779 |
| O | 1.7831247 | -1.2548525 | -2.4399649 |
| O | 3.0909721 | 0.3944606 | 1.0438550 |
| O | 0.9575056 | 2.6400242 | -1.6088793 |

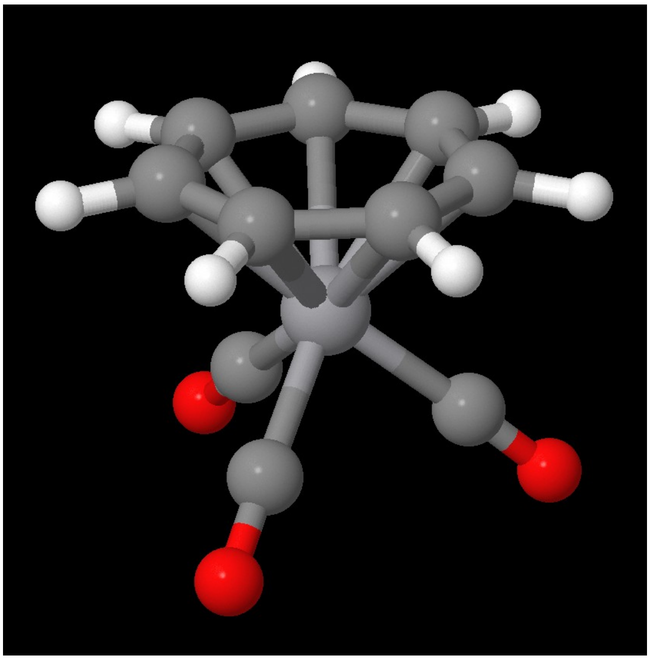

**$V(CO)_4C_5H_5$**

| | | | |
|---|---|---|---|
| 19 | | | |
| Atoms. | | | |
| V | -0.2243165 | -0.1709458 | 0.1203425 |
| C | 2.0379955 | -0.1224277 | 0.1147983 |
| C | 1.5906381 | 1.2176546 | 0.1082081 |
| C | 0.8650376 | 1.4325321 | -1.0827590 |
| C | -0.6804846 | 0.5111181 | 1.8542953 |
| C | -1.8643146 | 0.7857950 | -0.1501796 |
| H | 0.3917009 | 2.3543021 | -1.3762345 |
| H | 1.7658332 | 1.9464840 | 0.8815224 |
| H | 2.6210471 | -0.5905608 | 0.8897322 |
| C | 1.5872792 | -0.7397350 | -1.0778137 |
| C | 0.8604764 | 0.2253766 | -1.8183759 |
| H | 0.3914241 | 0.0694394 | -2.7749931 |
| C | -0.2087929 | -1.7060942 | 1.2655454 |
| C | -1.3873542 | -1.4297321 | -0.7340954 |
| H | 1.7727612 | -1.7582609 | -1.3735633 |
| O | -0.9548375 | 0.9160632 | 2.8928377 |
| O | -0.1974163 | -2.6288496 | 1.9487641 |
| O | -2.0812539 | -2.1858596 | -1.2491688 |
| O | -2.8475129 | 1.3559106 | -0.3123427 |

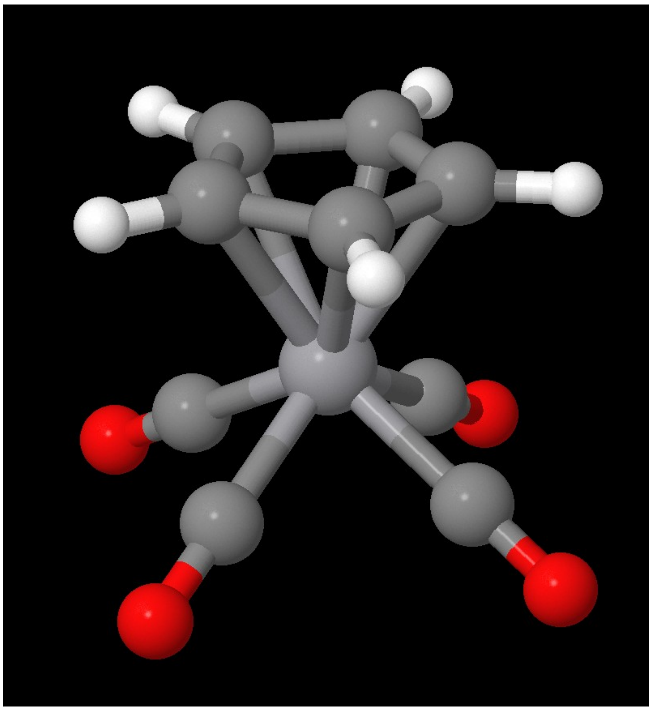

**$VF_5$**

```
6
Atoms.
V           0.0000000        0.0000016       -0.0000000
F           1.7423085       -0.0001912        0.0000000
F          -0.0000000        1.7060369        0.0000000
F          -1.7423085       -0.0001912        0.0000000
F          -0.0000000       -0.8528280        1.4775444
F          -0.0000000       -0.8528280       -1.4775444
```

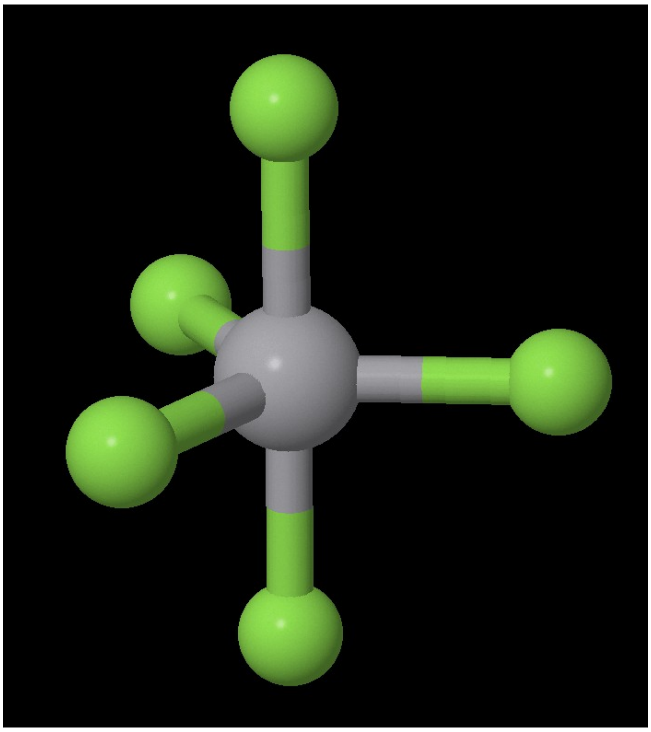

**$VOCl_3$**

```
5
Atoms.
O          0.0693199     -0.0004494     -0.0000000
V          1.6265902      0.0001084      0.0000000
Cl         2.3064328      2.0225793     -0.0000000
Cl         2.3059485     -1.0111191      1.7516667
Cl         2.3059485     -1.0111191     -1.7516667
```

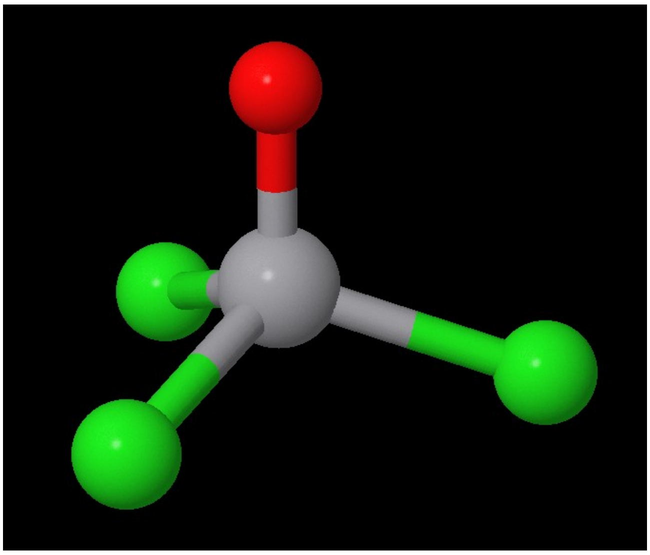

## $VOF_3$

```
5
Atoms.
O          -0.0091887       -0.0001270        0.0000000
V           1.5501047        0.0001952       -0.0000000
F           2.0996813        1.6271455        0.0000000
F           2.0995814       -0.8136069        1.4087456
F           2.0995814       -0.8136069       -1.4087456
```

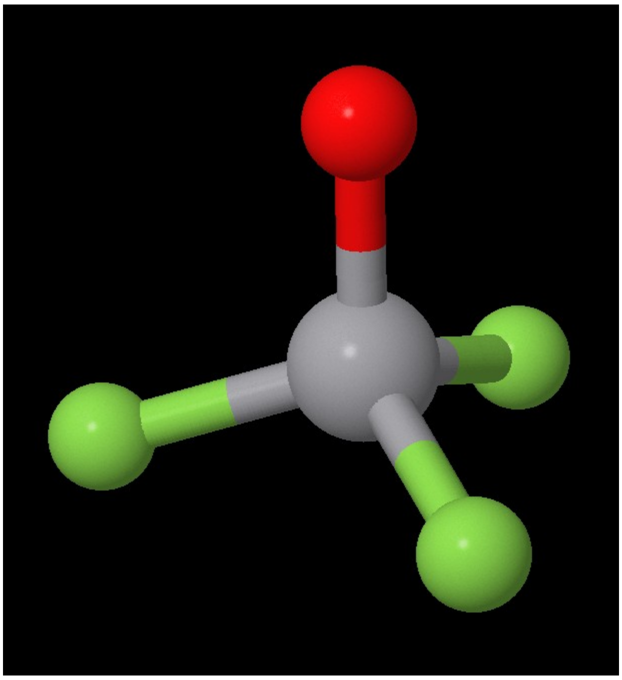

# Sample control.in files (excluding the definitions of basis sets) for $MnO_3Cl$

## Geometry optimization

```
xc                      dfauto scan
spin                    none
relativistic            atomic_zora scalar
sc_accuracy_rho         1.0e-7
sc_iter_limit           3000

relax_geometry          bfgs 0.005
```

## Ground state total energy

```
xc                      dfauto scan
spin                    collinear
default_initial_moment  0.0
relativistic            zora scalar 1e-12
sc_iter_limit           3000

KS_method               serial
restart_write_only      restart_file

override_illconditioning .true.
```

## Final state total energy

```
xc                      dfauto scan
spin                    collinear
default_initial_moment  0.0
relativistic            zora scalar 1e-12
sc_iter_limit           3000

KS_method               serial
restart_read_only       restart_file

override_illconditioning .true.

charge                  1.0

force_occupation_projector 4 1 0.0 4 6
```
